# Supplementary material for: Interpolation can hurt robust generalization even when there is no noise
Source: arXiv:2108.02883 source file (2021-12-16)
Supplement: Supplementary file 1 [file linreg_exp.tex]

\section{Linear regression - additional insights}
In this section we discuss how inconsistent adversarial training prevents interpolation for linear regression. We further highlight the relation between early stopping and ridge regularization when training with \iid{} isotropic Gaussian features.

\subsection{Inconsistent adversarial training}
\label{sec:linreg_inconsistent}

As shown in \cite{Javanmard20a} and using the same arguments as in Section~\ref{sec:linrobrisk},
the robust square loss under inconsistent perturbations
can be reformulated as
\begin{align*}
    \empriskrobunreg(\theta) &=
        \frac{1}{n} \sum_{i=1}^n (\vert\y_i - \langle x_i, \theta \rangle \vert + \epstrain \|\theta\|_2)^2
    \nonumber \\
    &=
    \frac{1}{n} \sum_{i=1}^n (y_i - \langle x_i, \theta \rangle )^2
    + \epstrain^2 \|\theta\|_2^2
    + \frac{2 \epstrain}{n}
    \|\theta\|_2 \sum_{i=1}^n \vert\y_i - \langle x_i, \theta \rangle \vert .
    \label{eq:linreg_robust_estimator}
\end{align*}

We only consider consistent adversarial training in the main text
since inconsistent perturbations prevent interpolation even when $d>n$,
that is $\empriskrobunreg(\theta)=0$ is unattainable for any $\eps > 0$.
Nevertheless we note that this optimization problem is equivalent to
$\ell_2$-regularized linear regression with $\lambda = \epstrain^2$
and an additional term involving both the weight norm and absolute
prediction residuals. We can observe this effect in Figure~4 of
\cite{Javanmard20a}.

%% As a result, inconsistent adversarial training
%% prevents the estimator from interpolating even in the
%% overparameterized regime where $d> n$.
% , the loss does not vanish and hence the estimator $\theathat$ cannot interpolate the train data.

%
% If the problem dimensionality $d$ is fixed and $\epstrain$ is large enough,
% the weight norm contributes more to the objective in
% \eqref{eq:linreg_robust_estimator} than the prediction residuals,
% which in turn prevents interpolation.
% We can observe this effect in Figure~4 of \cite{Javanmard20a}.
% However, while $\ell_2$-regularized linear regression simply mitigates overfitting
% around the interpolation threshold,
% the additional term in \eqref{eq:linreg_robust_estimator} yields a different behavior:
% overfitting is only partially mitigated and the interpolation threshold shifts
% towards larger degrees of overparameterization $d/n$.

\subsection{Ridge regularization vs. early stopping}
\label{sec:linreg_early_stopping}

For linear regression on isotropic features as studied in Section~\ref{sec:linreg}
there exists a well-known correspondence between
the optimization path of zero-initialized gradient descent
and the regularization path of the ridge regression estimator
(see for example \cite{Ali19,Ali20}).
Hence, Theorem \ref{thm:main_thm_lr} directly translates to
early stopped gradient descent on the mean squared loss.
%We refer to for the formal statement and proof of
%the equivalence \cite{Ali19,Ali20}.

% \ma{Just write that there is a 1:1 correspondence between early stopping
% and ridge regularization; cite corresponding paper.}
% \subsection{RO due to Implicit bias}
% \label{sec:linregl1}

% \subsection{Different effect on robust vs. standard risk}
% Due to different weighting
