# Supplementary material for: Interpolation can hurt robust generalization even when there is no noise
Source: arXiv:2108.02883 source file (2021-12-16)
Supplement: Supplementary file 2 [file logreg_exp.tex]

\section{Logistic regression - additional insights}
In this section we further discuss logistic regression studied in
Section \ref{sec:logreg}. In \suppmat{}~\ref{sec:inconsistent}, we
compare adversarial training with consistent and inconsistent attacks. Further, \suppmat{}~\ref{sec:gdlogreg} shows that early
stopping has a similar effect to ridge regularization and
\suppmat{}~\ref{sec:logregnoise} discusses how noise in the training
set can prevent the estimator from achieving a vanishing training
loss.  Consequently, adding noise unexpectedly leads to a lower robust
risk - compared to the robust max margin solution trained on noiseless
data.  Finally, for completeness, in \suppmat{}~\ref{sec:logreg_st_vs_at} we observe that
standard training with  ($\eps =
0$) does not exhibit overfitting, however do not discuss it in the
main text since it results in significantly worse standard and robust
prediction performance.

%% performance compared
%% to adversarial training for both the standard and robust risk, and hence
%% justify the focus on adversarial training in the main text.
%% We observe that overfitting does not occur for standard training
%% however sin

%% however, resulting in a significantly worse performance compared
%% to adversarial training for both the standard and robust risk.

\subsection{Inconsistent adversarial training}
\label{sec:inconsistent}

% \fy{i think story needs to be rewritten:
%   we argued we want no noise, but in high-dim whp and small enough
%   $\eps$ inconsistent is also no noise. but there's no difference asymptotically
%   for this choice of sequence of $\eps/\sqrt{d}$. write sth about this}

Many papers to date consider unrestricted (and hence inconsistent)
$\ell_p$-perturbations, that is choosing $\pertset{p}(\epsilon) = \{
\delta \in \R^d: \|\delta\|_p\leq \eps\}$ for both the training loss
\eqref{eq:ridgeloss} and robust evaluation \eqref{eq:AR}.  When
training with inconsistent perturbations however, it is possible that
the perturbed data crosses the true decision boundary and as a result,
forcing an interpolating solution to fit noise even when the actual
observations are noiseless.
%% Hence, inconsistent adversarial attacks may introduce some noise during training
%% even when the actual observations are noiseless.
Since we focus on consistent perturbations in the main text in order
to disentangle the effects of noise from finite-sample effects, we
do not discuss inconsistent perturbations there.

%% In this
%% section we show that in fact, consistent and inconsistent
%% perturbations during training in fact have indistinguishable population risks
%% \fy{probably just cause of our choice of $\eps$}
%we discuss inconsistent perturbations for completeness.

For completeness however, in
Figure~\ref{fig:logreg_inconsistent_vs_consistent}, we compare the
risks of (consistent) robust logistic regression estimators trained
with consistent and inconsistent $\ell_\infty$ perturbations, choosing
radius $\epstrain = 0.1$ for both training and evaluation.
%% For evaluation, the robust risk always uses consistent perturbations
%% of radius $\epstrain = 0.1$.
Interestingly, the performance of both the interpolator ($\lambda = 0$)
and the optimal regularized solution are similar
compared to the estimator trained with consistent attacks. This shows
that the effect of the inconsistency in the attacks for this choice of $n=1k$ and $\eps=0.1$ is only very
limited.

To investigate how the difference between consistent and inconsistent
adversarial training changes for different choices of $n,\eps$, we
plot in Figure
\ref{fig:logreg_inconsistent_vs_consistent_eps_increase} the risks of
the unregularized estimator ($\lambda \to 0$) with respect to the radius
of the attack $\eps$ for $d = 500$ and $n =200,1000$. While for small
$\eps$, both risks behave very similarly for both choices of $n$,
surprisingly, as $\eps$ grows, inconsistent adversarial training
performs better. In order to understand this phenomonon we depict the
robust (unregularized) logistic training loss in Figure
\ref{fig:logreg_inconsistent_vs_consistent_eps_increase_loss} which
shows that for larger $\eps$, the inconsistent adversarial estimator
in fact does not achieve a vanishing training loss.

Hence, we observe
that inconsistent perturbations induce noise that prevents interpolation
%% leads to implicit regularization preventing
%% interpolation
and thus effectively implicit regularization.
As a consequence, the population risk is lower for inconsistent
than for consistent training for large $\eps$.
%% leads to a better performance compared to
%% consistent adversarial training.
A similar effect can be observed when
adding explicit label noise, discussed in Section~\ref{sec:logregnoise}

\begin{figure}[htbp]
    \centering
    \begin{subfigure}[b]{0.48\textwidth}
        \centering
        \includegraphics[width=2.6in]{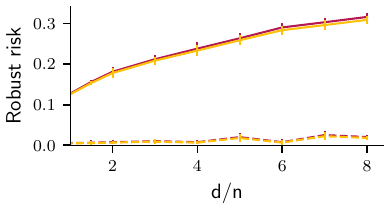}
        \caption{Consistent vs.~inconsistent adversarial training}
        \label{fig:logreg_inconsistent_vs_consistent_d_increase}
    \end{subfigure}
    \caption{ Comparison of logistic regression adversarial training
      with consistent and inconsistent $\ell_\infty$ perturbations.
      We simulate estimators from our data model for increasing
      degrees of overparameterization $d/n$ choosing $n=1000$ samples
      and $\epstrain = 0.1$ for both training and evaluation.
      The robust risk is calculated for consistent
      perturbations.  Since the setting is noisy, we average over five
      random dataset draws and use error bars to mark standard
      deviations.  While the estimators trained with inconsistent
      perturbations exhibit a slightly larger robust risk compared to
      estimators trained with consistent perturbations, the difference
      in both the interpolating ($\lambda \to 0$) and optimally
      $\ell_2$-regularized case is negligible.
        %\fy{i don't get that sentence}
        %Hence, overfitting must have a different explanation.
    }
    \label{fig:logreg_inconsistent_vs_consistent}
\end{figure}

\begin{figure*}[htbp]
    \centering
    \begin{subfigure}[b]{0.48\textwidth}
        \centering
        \includegraphics[width=2.6in]{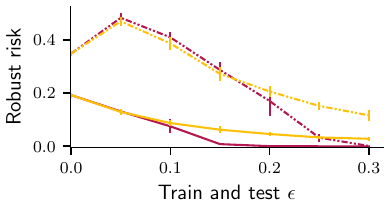}
        \caption{Varying $\eps$ for different $n$}
        \label{fig:logreg_inconsistent_vs_consistent_eps_increase}
    \end{subfigure}
        \begin{subfigure}[b]{0.48\textwidth}
        \centering
        \includegraphics[width=2.6in]{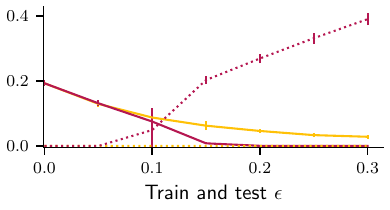}
        \caption{Robust risk vs.~training loss}
        \label{fig:logreg_inconsistent_vs_consistent_eps_increase_loss}
    \end{subfigure}
    \caption{ Comparison of logistic regression adversarial training
      with consistent vs. inconsistent $\ell_\infty$ perturbations. a)
      For fixed $d=500$, we plot the robust risks for $n=200, 1000$,
      of the unregularized  estimators $(\lambda \to 0)$ with respect to
      $\eps$. While for small $\eps$, adversarial training with both
      consistent and inconsistent yield similar robust risks, for
      large $\eps$, inconsistent attacks yield a better
      performance. In b) we give an explanation for the observation in
      (a) by additionally plotting the training loss of the
      unregularized estimator as a function of $\eps$ for fixed $n
      =1000$, $d=500$. We observe that, in contrast to training with
      consistent attacks, unregularized ($\lambda \to 0$) inconsistent
      adversarial training does not achieve vanishing training loss
      when increasing $\eps$ and is hence implicitly regularized. }
    \label{fig:logreg_inconsistent_vs_consistent_2}
\end{figure*}

% overfitting gap does
% not change significantly, showing that the inconsistent attacks are not harmful
% and achieve a very similar performance to the training with consistent attacks.
% Hence, overfitting must have a different explanation.

%
% We use $n=1000$ samples from our data model and varying degrees of overparameterization $d/n$
% for the simulation and compare interpolating estimators ($\lambda = 0$)
% to their optimally $\ell_2$-regularized counterparts.
% Since inconsistent perturbations induce noise,
% we average over five random dataset draws and use error bars
% to mark standard deviations.
% Surprisingly, the overfitting gap does
% not change significantly, showing that the inconsistent attacks are not harmful
% and achieve a very similar performance to the training with consistent attacks.
% Hence, overfitting must have a different explanation.

\subsection{Ridge regularization vs. early stopping}
\label{sec:gdlogreg}
Throughout Section~\ref{sec:logreg}, we exclusively focus on
$\ell_2$-regularized estimators.  While there is a one-to-one
correspondence between $\ell_2$-regularization and early stopping in
the linear regression case (see
Section~\ref{sec:linreg_early_stopping}), we are not aware of similar
results for logistic regression.  In this section, we provide
experimental evidence that early stopped gradient descent, similar to
$\ell_2$-regularization, can benefit the robust risk for logistic
regression.

Figure~\ref{fig:logreg_early_stopping} shows simulation results on our
synthetic data model for $n=1000$ training samples and
overparameterization ratio $d/n = 8$.  We use consistent $\ell_\infty$
perturbations of radius $\eps = 0.1$ for both the robust loss
$\empriskrob$ during training and for the robust risk $\AR$.  For
Figure~\ref{fig:logreg_early_stopping_gd}, we run zero-initialized
gradient descent on the unregularized loss ($\lambda = 0$) for $500k$
iterations whereas in Figure~\ref{fig:logreg_early_stopping_regularized}, we minimize the loss with respect to a series of
decreasing $\lambda$ using a convex programming solver.  We observe robust
overfitting over time with the following learning rate schedule:
%In order to observer an initial decrease \fy{weird} of the robust risk,
we use a small initial step size of $0.01$ and
%accelerate convergence towards the max-margin interpolator by
double the step size every $30k$ steps until iteration $300k$.

\begin{figure*}[htbp]
    \centering
    \includegraphics[width=5.5in]{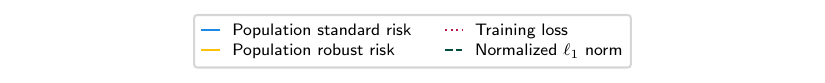}
    \begin{subfigure}[b]{0.48\textwidth}
        \centering
        \includegraphics[width=2.6in]{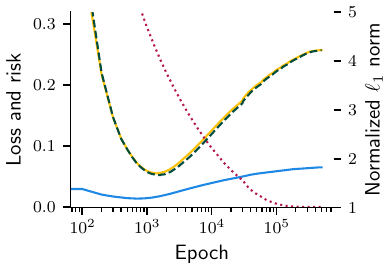}
        \caption{Gradient descent}
        \label{fig:logreg_early_stopping_gd}
    \end{subfigure}
    \begin{subfigure}[b]{0.48\textwidth}
        \centering
        \includegraphics[width=2.6in]{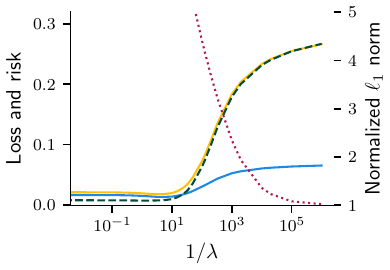}
        \caption{$\ell_2$-regularization}
        \label{fig:logreg_early_stopping_regularized}
    \end{subfigure}
    \caption{ Trends for unregularized gradient descent and varying
      $\lambda$.  We simulate robust logistic regression estimators
      with respect to consistent $\ell_\infty$ perturbations of radius
      $\eps = 0.1$ for both training and evaluation using $n=1000$
      training samples of our synthetic data model with
      overparameterization ratio $d/n = 8$.  We plot the population risks,
      robust logistic loss on the training data (training loss)
      for (a) gradient descent iterates on the unregularized robust loss for $\lambda = 0$ and (b) for $\ell_2$-regularized estimators for increasing
      $1/\lambda$. We observe that both early stopping and optimal $\ell_2$
      regularization prevent interpolation and yield a significantly
      smaller robust risk compared to the estimator with vanishing
      robust logistic loss. Furthermore the
    interpolating estimators are more dense than at the optimal stopping time or choice of $\lambda$ respectively. }
    \label{fig:logreg_early_stopping}
\end{figure*}

% resulting
% in the max-margin solution \fy{how do we know its the max margin?}.

Evidently, both early stopping and $\ell_2$-regularization prevent
interpolation and yield an estimator with significantly lower standard
and robust risk compared to the interpolator ($\lambda \to 0$)
respectively converged estimator (gradient steps $\to
\infty$)\footnote{For standard logistic regression gradient descent
  converges in the direction of the max margin solution
  \cite{Ji19}. We therefore also conjecture that gradient descent on
  the unregularized robust loss \eqref{eq:AR} converges in the
  direction of the peanlized max margin estimator
  \eqref{eq:maxmarginAE}. We leave this as a future work.}.  We
further observe in both cases that the estimator becomes increasingly
less sparse (measured by the $\ell_1 / \ell_2$ ratio which we refer to
as normalized $\ell_1$ norm) as the training loss starts to vanish.
However, explicit $\ell_2$-regularization seems to yield better
quantities overall.

%  \fy{if you add vertical lines, you
%   can focus on the point past ``0-1 interpolation'' and don't have to discuss the first descent}
%% Note that for gradient descent, the robust risk decreases significantly during the first
%% training iterations before reaching its minimum value,
%% while Figure~\ref{fig:logreg_early_stopping_regularized}
%% seems to suggest that even very large $\lambda$ values result in an almost optimal robust risk.
%% Nonetheless, if $\lambda$ is large enough, the resulting $\ell_2$-regularized estimator
%% is close to zero, yielding a similar curve as in Figure~\ref{fig:logreg_early_stopping_gd}.
%% However, the corresponding optimization problem is numerically unstable and
%% we hence omitted it from the plot.

\begin{figure*}
    \centering
    \begin{subfigure}[b]{0.48\textwidth}
        \centering
        \includegraphics[width=2.6in]{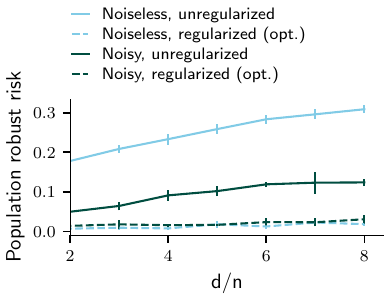}
        \caption{Effect of label noise and regularization}
        \label{fig:logreg_noise_levels}
    \end{subfigure}
    \begin{subfigure}[b]{0.48\textwidth}
        \centering
        \includegraphics[width=2.6in]{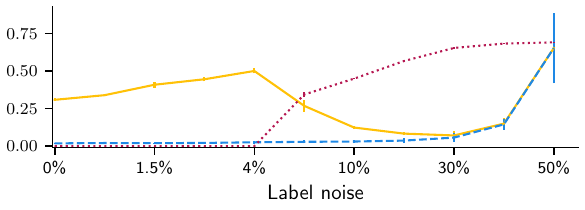}
        \caption{Varying label noise}
        \label{fig:logreg_noise_increase}
    \end{subfigure}
    \caption{ a) Difference between training robust logistic
      regression estimators with 0\% and 10\% label noise.  We
      minimize the robust loss on $n=1000$ samples from our synthetic
      data model for varying degrees of overparameterization $d/n$ and
      use consistent $\ell_\infty$ perturbations of radius $\epstrain
      = 0.1$ for both training and evaluation.  Since the setting is
      noisy, we average over five random dataset draws and use error
      bars to mark standard deviations.
      %% The plots show the training
      %% loss and robust risk for estimators without regularization and
      %% with optimal $\ell_2$-regularization.
      b) The training loss and
      the robust and standard risk of the unregularized estimator
      $(\lambda \to 0$) with respect to the percentage of clean labels in
      the training dataset for $\eps =0.1$, $n =1000$ and $d=8000$.
      We observe that, counterintuitively, noisy training data yields
      estimators with lower robust risk since the label noise prevents
      interpolation.  However, as soon as we apply regularization,
      the spurious benefits of label noise vanish, and clean training
      data yields estimators with equal or better robust risk compared
      to noisy data.  }
    \label{fig:logreg_noise}
\end{figure*}

\subsection{Noisy adversarial training as regularization}
\label{sec:logregnoise}

Instead of preventing interpolation via regularization, we now
consider the case where we introduce significant noise by flipping
$10\%$ of the training labels.  When the percentage of label flips and
the radius $\epstrain$ for consistent perturbations are large enough,
the max-margin estimator \eqref{eq:maxmarginAE} does not exist.  As a
consequence, the estimator that we obtain by minimizing the
adversarially robust logistic loss \eqref{eq:logridge} does not
interpolate and we effectively obtain a regularized estimator.
% via adversarial training with sufficient noise.

Figure~\ref{fig:logreg_noise_levels} compares the final robust risk on
noiseless samples to the robust risk on data with 10\% label noise for
unregularized training. %($\ynoisestd = 0.1$).  As expected from
classical theory, for a non-zero ridge penalty and both noisy and
noiseless adversarial training converge to the same solution. However, in
contrast to the usual intuition that noise in the training data hurts
the performance,
%especially when regularization is absent,
%we actually observe in Figure~\ref{fig:logreg_noise_levels_interpolating}
we observe that across overparameterization ratios, the robust risk
of the unregularized estimator trained on noisy data is lower. 

In order to understand this phenomenon,
Figure~\ref{fig:logreg_noise_increase} shows the robust and standard
risk together with the robust $0-1$ loss on the training data as a
function of the percentage of correct labels in the training
set. Starting from 100\% clean labels, adding noisy labels in the
dataset initially increases the risk of the estimator as
expected. When further increasing the percentage of clean samples
however, the estimator loses the ability to achieve vanishing training
loss, effectively leading to implicit regularization.  Indeed, at this
point the risk starts to decrease again. In particular, training on
the data with $20\%$ label flips results in a robust risk that is
$\sim 25\%$ lower than training on the clean dataset without any
mislabeled samples. In brief, label noise mitigates interpolation and
hence leads to implicit regularization.

Finally, we remark that the from a practical point of view, this
section does not motivate to add artificial label noise to the
training dataset, but motivates the use of regularization.

% 
% after a certain threshold the estimator does no longer achieve a vanishign train loss. 
% 

%% While this clearly leads to the misleading conclusion that adding
%% label noise helps to improve performance, we can actually observe that
%% the noise in the training data shifts the interpolation threshold of
%% the adversarially perturbed training data set towards larger
%% $d/n$. \fy{this is not shown in this plot, theres no interpolation for
%%   noisy, also here in legend training loss is again misleading -> with
%%   $\lambda$ term or not} This is accentuated by
%% Figure~\ref{fig:logreg_noise_levels_regularized} which shows that
%% explicit $\ell_2$-regularization yields a smaller robust risk for both
%% noisy and noiseless data when compared to the unregularized case.
%% \fy{don't understand}

\subsection{Standard vs. adversarial training}
\label{sec:logreg_st_vs_at}

While we focus on adversarial training for logistic regression
throughout this paper as it achieves much higher standard and robust
accuracy in our model, we also provide simulation results for standard
training (that is $\epstrain=0$) in
Figure~\ref{fig:logreg_standard_training} for completeness.  We again
use a dataset of size $n=1000$.  In contrast to adversarial training
with $\epstrain > 0$, we do not observe overfitting for neither the
standard nor robust risk.  In particular, for $d > n$, the robust risk
exhibits its maximum possible value.  Our observations are consistent
with \cite{Salehi19}.

\begin{figure*}[htbp]
    \centering
    \includegraphics[width=2.6in]{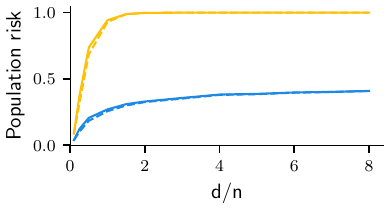}
    \caption{
        Simulated standard training risks of logistic regression estimators for
        varying degrees of overparameterization $d/n$
        using $n=1000$ training samples from our synthetic data model.
        While we do not observe any overfitting,
        the robust risk quickly deteriorates to its maximum value as soon as $d > n$.
    }
    \label{fig:logreg_standard_training}
\end{figure*}
