# Supplementary material for: Interpolation can hurt robust generalization even when there is no noise
Source: arXiv:2108.02883 source file (2021-12-16)
Supplement: Supplementary file 3 [file logreg_theory_.tex]

\section{Logistic regression - theory}
\label{appendix:logreg}

Some definitions, we let $\Moureau_f(\x,t) = \min_{y} \frac{1}{2t}(x-y)^2 + f(y)$ be the Moureau envelope. Further, define $Z$ to be the standard normal Gaussian random variable and $Z_{\sigma} = \left\{\begin{matrix}~~~~~~ \vert Z \vert ~~w.p.~~ 1-\sigma \\ - \vert Z \vert ~~w.p.~~ \sigma \end{matrix} \right.$.

\begin{lemma}
\label{lm:logregrisk}
The population standard and robust risk from Equation \eqref{eq:SR},\eqref{AR} can be expressed as
 \begin{align}
 \SR &= \frac{1}{\pi}\arccos\left(\frac{\langle\thetanull,\thetahat\rangle}{\|\thetahat\|_2}\right) ~~\mathrm{and}~~
  \AR = \frac{1}{\pi}\arccos\left(\frac{\langle\thetanull, \thetahat\rangle}{\|\thetahat\|_2}\right) + 2\Phi(t/\sqrt{2}) + 2I\left(t, \frac{\langle\thetanull,\thetahat\rangle}{\|\thetahat\|_2}\right)
\end{align}
with $t \define \frac{\epstest(\|\thetahat\|_q^q -\langle \thetanull,\thetahat\rangle)^{1/q}}{\|\thetahat\|_2}$ and $q$ such that $\frac{1}{p} +\frac{1}{q} = 1$ and 
\begin{equation}
 I(t,u) \define \int_{0}^{t} \frac{1}{2\sqrt{2\pi}}\Phi\left(\frac{x u}{\sqrt{2}\sqrt{1- u^2}}\right) \exp\left(-\frac{x^2}{2}\right)dx  
\end{equation}
\end{lemma}

We are going to make use of the following well known facts on the derivative of the Moreau envelope \kd{wrong citation:}(e.g. see Appendix A in\cite{Ali20}):
\begin{align}
\frac{\partial \Moureau_{f}(x,t)}{\partial x} &= \frac{1}{t}(x - \Prox_f(x,t))
\label{eq:moreau1}
\\
\frac{\partial \Moureau_{f}(x,t)}{\partial t} &= -\frac{1}{2t^2}(x - \Prox_f(x,t))^2
\label{eq:moreau2}
\end{align}
where $\Prox_f(x,\mu)$ is the proximal operator \kd{need citation}:
\begin{equation}
 \Prox_f(x,\mu) = \arg\min_{t} f(t) + \frac{1}{2\mu}(t-x)^2.
\end{equation}

\begin{prop}
  \label{prop:gammastar}
  about $\gammastar$
\end{prop}

\subsection{Non separable regime}

\begin{theorem}
\label{thm:consistentnonsep}
 Assume that $\gamma \leq \gammastar$ and $\lambda = 0$ or $\lambda > 0$. Furthermore, assume that $\eps = \eps_0/\sqrt{d}$.  $(\nuper^\star,\nupar^\star, \otaur^\star, \otaul^\star, \orv^\star,\odelta^\star,\mu^\star)$ be the unique solution of
 \begin{equation}
 \begin{split}
 \label{eq:nonseperable}
  \min_{\substack{\nuper\geq 0, \otaul\geq 0 \\ \nupar, \odelta \geq 0}}\max_{\substack{r, \mu\geq 0}} ~ &\EE_{\Zrv_{\sigma},\Zrv}\left[ \Moureau_{\lossf}(\Zrv_{\sigma}\nupar + \Zrv \nuper - \eps_0 \odelta, \frac{\otaul}{\orv})\right]  - \odelta \mu +\frac{\orv \otaul}{2} + \lambda(\nuper^2 +\nupar^2) \\
%       -\odelta&\EE_{\Zrv}\left[ \Moureau_{\vert.\vert}(\orv \sqrt{\gamma} \Zrv, \frac{\otaur\odelta}{\nuper})\right]
      -&\nuper \sqrt{\left[ (\mu^2+\gamma\orv^2) -  (\mu^2+\gamma\orv^2) \erf(\mu/(\sqrt{\gamma}\orv\sqrt{2})) - \sqrt{\frac{2}{\pi}} \sqrt{\gamma}\orv\mu \exp(-\mu^2/(\gamma \orv^2 2)) \right]} 
      \end{split}
 \end{equation}
 then asympototiclally as $d/n \to \gamma$, we have that 
 \begin{align}
  \|\thetahat_{\perp} \|_1  &\to \odelta \\
  \langle \thetahat,  \thetanull \rangle &\to \nupar \\
  \|\thetahat\|_2^2 &\to \nupar^2 + \nuper^2 
 \end{align}
 \kd{now we also need to add the inconsistent perturbations...}
\end{theorem}

We note that we can use this theorem to derive a fixed point problem. \kd{too tired to write more here}. For this, let $\partial_x \Moureau_l$ denote the derivative given in Equation \eqref{eq:moreae1}
and $\partial_{t} \Moureau_l$ the derivative from Equation \eqref{eq:moreau2}. For compactness, we write $\EMoureau = \EE_{\Zrv_{\sigma},\Zrv}\left[ \Moureau_{\lossf}(\Zrv_{\sigma}\nupar + \Zrv \nuper - \eps \odelta, \frac{\otaul}{\orv})\right]$ and denote with $\EMoureau_{\nupar} = \EE_{\Zrv_{\sigma},\Zrv}\left[ \partial_x \Moureau_{\lossf}(\Zrv_{\sigma}\nupar + \Zrv \nuper - \eps \odelta, \frac{\otaul}{\orv}) \frac{\partial (\Zrv_{\sigma}\nupar + \Zrv \nuper - \eps \odelta)}{\partial \nuper}\right]$ the derivative of the expected Moreau envelope with respect to $\nupar$ and similar for the other varables. Further, for simplicity, define $\expterms =  (\mu^2+\gamma\orv^2) -  (\mu^2+\gamma\orv^2) \erf(\mu/(\sqrt{\gamma}\orv\sqrt{2}))- \sqrt{\frac{2}{\pi}} \sqrt{\gamma}\orv\mu \exp(-\tilde{\mu}^2/2)$ and denote with $ g_{\mu}$ respectively $g_{\orv}$ the corresponding partial derivatives. 

% \begin{cor}
% \label{cr:nonsepfixedpoint}
% Too lazy to state the equations here, just take a look at the proof. 
% \end{cor}
% 

\subsubsection{Proof of Theorem \ref{thm:consistentnonsep}}

 The goal is to asympototically to study the solution of the following optimization problem
\begin{equation*}
 \thetahat = \arg\min_{\theta} \frac{1}{n} \sum_{i = 1}^{n} \lossf(\y_i \langle x_i, \theta \rangle - \eps  \|\theta_{\perp}\|_1) + \lambda \|\theta\|_2^2
\end{equation*}
where $\lossf(x) = \log(1+\exp(-x))$ is the logistic loss. 
Using the same argument as \cite{Javanmard20}, this problem is equivalent to 
\begin{equation*}
 \min_{\theta,v} \max_{u} ~\frac{1}{n} \sum_{i=1}^{n} \lossf(v_i - \eps \|\theta_{\perp}\|_1) + \frac{1}{n} u^\top \Dy \Xs \theta - \frac{1}{n} u^\top v+ \lambda \|\theta\|_2^2,
\end{equation*}
where $\Dy$ is the diagonal matrix with entries $(\Dy)_{i,i} = \y_i$. Next, define $\Hone = \Xs \Pi_{\parallel}$ and $\Htwo = \Xs \Pi_{\perp}$. We can write
\begin{equation*}
 \min_{\theta,v} \max_{u} ~ \frac{1}{n} \sum_{i=1}^{n} \lossf(v_i - \eps \|\theta_{\perp}\|_1) + \frac{1}{n} u^\top \Dy \Hone \thetapar + \frac{1}{n} u^\top \Dy \Htwo \thetaper - \frac{1}{n} u^\top v + \lambda \|\theta\|_2^2.
\end{equation*}
Because $\Htwo$ is independent of the observations $\y$ and of $\Hone$, this allows us to apply the Convex Gaussian Minimax Theorem. As a result, we converge asymptotically to the same solution as 
\begin{equation*}
 \min_{\theta,v} \max_{u} ~ \frac{1}{n} \sum_{i=1}^{n} \lossf(v_i - \eps \|\theta_{\perp}\|_1) + \frac{1}{n} u^\top \Dy \Hone \thetapar +\frac{1}{n} \|u^\top \Dy\|_2 g^\top \thetaper +\frac{1}{n} u^\top \Dy h \| \thetaper \|_2  - \frac{1}{n} u^\top v + \lambda \|\theta\|_2^2,
\end{equation*}
where $g\in\RR^p$ and $h\in \RR^n$ are vectors i.i.d. standard normal distributed entries. The goal is now to find an asymptotically equivalent low dimensional optimization problem.   

In a first step, we maximize over $u$. For this, define $\orv =  \|u\|_2/\sqrt{n}$, which allows us to equivalently write:
 \begin{equation*}
 \min_{\theta,v} \max_{\orv \geq 0} ~ \frac{1}{n} \sum_{i=1}^{n} \lossf(v_i - \eps \|\theta_{\perp}\|_1) + \frac{r}{\sqrt{n}} \|\Dy \Hone \thetapar  + \Dy h \| \thetaper \|_2  -  v \|_2 +\frac{1}{\sqrt{n}} \orv g^\top \thetaper + \lambda \|\theta\|_2^2,
\end{equation*}
where we have used the fact that $\|u^\top \Dy\|_2 = \|u\|_2$. Next, we note that because the problem is convex in $\orv$ and concave in $\theta,v$, we can swap maximization with minimization. In order to proceed, we want to separate $\thetaper$ form the loss $\lossf(v,\thetaper)$. For this, note that we can write $\lossf(v,\thetaper) = \frac{1}{n} \sum_{i=1}^{n} \lossf(v_i - \eps \|\theta_{\perp}\|_1)$ in terms of its conjugate with respect to $\thetaper$: 
\begin{equation}
 \lossf(v,\thetaper) = \sup_{w} \frac{1}{\sqrt{d}}w^\top  \thetaper - \conjlossf(v,w),
\end{equation}
where $\conjlossf$ is the conjugate of $\lossf$. In particular, we can use Lemma A.2 in the paper \cite{Javanmard20} which shows that
\begin{equation}
 \conjlossf(v,w) = \sup_{\odelta \geq 0} \frac{\sqrt{d}}{\sqrt{d}}\odelta \|w\|_{\infty} - \frac{1}{n} \sum_{i=1}^n \lossf(v_i - \sqrt{d}\eps \odelta) = \sup_{\odelta \geq 0} \odelta \|w\|_{\infty} - \frac{1}{n} \sum_{i=1}^n \lossf(v_i - \eps_0 \odelta)
\end{equation}
Hence we can write
\begin{align}
 \max_{r\geq 0,w} \min_{\theta,v,\odelta\geq0} \frac{1}{n} \sum_{i=1}^n \lossf(v_i - \eps_0 \odelta)  + \frac{1}{\sqrt{d}}w^\top \thetaper - \odelta \|w\|_{\infty}   + \frac{r}{\sqrt{n}} \|\Dy \Hone \thetapar  + \Dy h \| \thetaper \|_2  -  v \|_2 +\frac{1}{\sqrt{n}} \orv g^\top \thetaper + \lambda \|\theta\|_2^2.
\end{align}
We can now simplify the optimization over $\theta$. First, note that we can with $\thetapar = \Pipar 1 \nupar$ where $\nupar \in \RR$. Further, let $\nuper = \|\thetaper\|_2$. We can then solve the inner maximization over $\theta$ by
\begin{align}
 \max_{r\geq 0,w} \min_{\nuper \geq 0, \nupar,v,\odelta\geq0} &\frac{1}{n} \sum_{i=1}^n \lossf(v_i - \eps_0 \odelta) 
 - \frac{1}{\sqrt{d}}\nuper \| \Piper(w - \sqrt{\gamma} \orv g)\|_2 \\ -&\odelta \|w\|_{\infty}   + \frac{r}{\sqrt{n}} \|\Dy \Hone \Pipar 1 \nupar  + \Dy h \nuper  -  v \|_2  + \lambda (\nupar^2 +\nuper^2).
\end{align}
In order to further proceed, we need to repalce the term $ \|\Dy \Hone \Pipar 1 \nupar  + \Dy h \nuper  -  v \|_2 $ with their squares. This is achieved by using the following identitiy $\min_{\tau\geq0} \frac{x^2}{2\tau} + \frac{\tau}{2} = x$. 
Hence, we can write 
\begin{align}
 \max_{r\geq 0,w} \min_{\nuper \geq 0, \nupar,v,\odelta\geq0, \otaul\geq 0} &\frac{1}{n} \sum_{i=1}^n \lossf(v_i - \eps_0 \odelta) 
 - \nuper \frac{1}{\sqrt{d}}\| \Piper(w - \sqrt{\gamma} \orv g)\|_2 - \frac{\nuper\otaur}{2}
 \\ -&\odelta \|w\|_{\infty}   + \frac{\orv}{2\otaul n} \|\Dy \Hone \Pipar 1 \nupar   + \Dy h \nuper  -  v \|_2^2+ \frac{\otaul \orv}{2}  + \lambda (\nupar^2 +\nuper^2),
\end{align}
where we have used again the fact that we can interchange the maximum and minimum due to the convexity respectivity concavity of the objective. 
We can now seperately solve the following two inner optimization problems:
\begin{align}
 &\max_{w}~ - \frac{\nuper}{2\otaur}\frac{1}{d}\| \Piper(w - \sqrt{\gamma} \orv g)\|_2^2  -\odelta \|w\|_{\infty} \\
 &\min_{v}~ \frac{\orv}{2\otaul n} \|\Dy \Hone \Pipar 1 \nupar +  \Dy h \nuper  -  v \|_2^2 +  \sum_{i=1}^n \lossf(v_i - \eps_0 \odelta) 
\end{align}
\paragraph{Term 1}
We begin with the first equaton. Let $\SoftT_t(x) = \left\{\begin{matrix} 0 ~\abs{x} \leq t \\ \sgn(x)(\abs{x}-t) ~\mathrm{else}                                                         
\end{matrix}\right. $ be the soft thresholding function. We can now maximize over $w$: 
\begin{align}
 &\max_{w}~ -\frac{\nuper}{2\otaur} \frac{1}{\sqrt{d}}\| \Piper(w - \sqrt{\gamma} \orv g)\|_2  -\odelta \|w\|_{\infty} \\
 = - &\min_{w}~  \frac{\nuper}{2\otaur}\frac{1}{\sqrt{d}}\| \Piper(w - \sqrt{\gamma} \orv g)\|_2  -\odelta \|w\|_{\infty} \\ 
 \overset{\mu = \|w\|_{\infty}}{=} -&\min_{\mu \geq0} \frac{\nuper}{2\otaur}~ \sqrt{ \frac{1}{d} \sum_{i=2}^d \left(\SoftT_{\mu}\left(\sqrt{\gamma} \orv g_i\right)\right)^2} +\odelta \mu \\
  \overset{\mathrm{LLN~as~} d\to \infty}{\to} -&\min_{\mu \geq0} \frac{\nuper}{2\otaur}~ \sqrt{\EE_Z \left(\SoftT_{\mu}\left(\sqrt{\gamma} \orv Z \right)\right)^2} +\odelta \mu 
\end{align}
For simplicity, define $\alpha = \sqrt{\gamma}r$ and $\tilde{\mu} = \mu/\alpha$. We have
\begin{align}
 \EE_Z \left(\SoftT_{\mu}\left(\sqrt{\gamma} \orv Z \right)\right)^2 &= \alpha^2 \EE_Z \left(\SoftT_{\tilde{\mu}}\left( Z \right)\right)^2 \\
 &= \alpha^2 \EE_Z (Z- \tilde{\mu})^2 - \EE_Z \indicator_{\abs{Z} \leq \tilde{\mu}} (Z- \tilde{\mu})^2 \\
 &= \alpha^2 (\tilde{\mu}^2+1) - \alpha^2 (\tilde{\mu}^2+1) \erf(\tilde{\mu}/\sqrt{2})- \alpha^2 \sqrt{\frac{2}{\pi}} \tilde{\mu} \exp(-\tilde{\mu}^2/2)
\end{align}

\paragraph{Term 2}
For the second term we can use a similar argument: 
\begin{align}
  &\min_{v}~ \frac{\orv}{2\otaul n} \|\Dy \Hone \Pipar 1 \nupar  + \Dy h \nuper  -  v \|_2^2 +  \frac{1}{n}\sum_{i=1}^n \lossf(v_i - \eps_0 \odelta) \\
  \overset{\tildev = v - \eps\odelta}{=} &\min_{\tildev}~  \frac{\orv}{2\otaul n} \|\Dy \Hone \Pipar 1 \nupar +  \Dy h \nuper  -  \tildev - \eps_0 \odelta \|_2^2 +  \frac{1}{n} \sum_{i=1}^n \lossf(\tilde{v}_i) \\
  \overset{\mathrm{LLN}}{\to} &~~\EE_{\Zrv_{\sigma},\Zrv}\left[ \Moureau_{\lossf}(\Zrv_{\sigma}\nupar + \Zrv \nuper - \eps_0 \odelta, \frac{\otaul}{\orv})\right].
\end{align}
For the last line, we remark that $(\Dy\Hone \Piper1)_i = \y_i\x_i^\top\thetanull = \xi_{\sigma}\sgn(\x_i^\top\thetanull) \x_i^\top\thetanull$ which has the same distrubtion as $\Zrv_{\sigma}$. We can then apply the law of large numbers because \kd{say something again...}.
Combining these results, we then obtain the optimization problem which completes the proof of the theorem. 
\qed

\subsubsection{Proof of Corollary \ref{cr:nonsepfixedpoint}}
Since the problem in Theorem \ref{thm:consistentnonsep} is convex-convave, we know that a solution may be found which does not lie on the boundary if and only if $\nabla C = 0$ where $C$ is the optimization objective. For training with consistent perturbations, we have 
\begin{align}
  C =  \EMoureau - &\nuper \sqrt{g(\mu,\orv)} - \odelta \mu 
       +\frac{\orv \otaul}{2} + \lambda(\nuper^2 +\nupar^2)
\end{align}
Taking the derivative this gives us
\begin{align}
0 &= \frac{\partial }{\partial \nupar} C = \EMoureau_{\nupar} + 2\lambda \nupar\label{eq:Cnonsep1} \\
0 &= \frac{\partial }{\partial \nuper} C = \EMoureau_{\nuper} + 2\lambda \nuper -\sqrt{g}\label{eq:Cnonsep2}\\
0 &= \frac{\partial }{\partial \otaul} C = \EMoureau_{\otaul} + \frac{r}{2} \label{eq:Cnonsep4} \implies &\orv = -2\EMoureau_{\otaul}\\
0 &= \frac{\partial }{\partial \odelta} C = \EMoureau_{\odelta} - \mu \label{eq:Cnonsep5} \implies &\mu = \EMoureau_{\delta}\\
0 &= \frac{\partial }{\partial \mu} C =-\frac{\nuper}{2 \sqrt{g}} g_{\mu} - \delta \label{eq:Cnonsep6} \implies & \delta = -\frac{\nuper}{2\sqrt{g}} g_{\mu}\\
0 &= \frac{\partial }{\partial \orv} C = \EMoureau_{\orv} -\frac{\nuper}{2\sqrt{g}} g_{\orv} + \frac{\otaul}{2}\label{eq:Cnonsep7} \implies &\otaul = -2\EMoureau_{\orv} + \frac{\nuper}{\sqrt{g}}g_{\orv}
\end{align}
Furthermore, note that 
\begin{align}
 \EMoureau_{\nuper} &= \EE_{\Zrv_{\sigma},\Zrv}\left[ \frac{\orv}{\otaul}(\Zrv_{\sigma}\nupar + \Zrv \nuper - \eps \odelta -  \Prox_{\lossf}(\Zrv_{\sigma}\nupar + \Zrv \nuper - \eps \odelta, \frac{\otaul}{\orv})) \Zrv \right] \\
 &=  \frac{\orv}{\otaul} \nuper - \EE_{\Zrv_{\sigma},\Zrv}\left[ \frac{\orv}{\otaul}( \Prox_{\lossf}(\Zrv_{\sigma}\nupar + \Zrv \nuper - \eps \odelta, \frac{\otaul}{\orv})) \Zrv \right] \\
\end{align}
and hence
\begin{equation}
\nuper = \EE_{\Zrv_{\sigma},\Zrv}\left[( \Prox_{\lossf}(\Zrv_{\sigma}\nupar + \Zrv \nuper - \eps \odelta, \frac{\otaul}{\orv})) \Zrv \right] -  \frac{\otaul}{\orv}\left(2\lambda\nuper - \sqrt{g} \right).
\end{equation}
Finally, we have
\begin{align}
  \EMoureau_{\nupar} &= \EE_{\Zrv_{\sigma},\Zrv}\left[ \frac{\orv}{\otaul}(\Zrv_{\sigma}\nupar + \Zrv \nuper - \eps \odelta -  \Prox_{\lossf}(\Zrv_{\sigma}\nupar + \Zrv \nuper - \eps \odelta, \frac{\otaul}{\orv})) \Zrv_{\sigma} \right] \\
 &=  \frac{\orv}{\otaul} \nupar \EE_{\Zrv_{\sigma}} \Zrv_{\sigma}^2 - 
 \frac{\orv}{\otaul} \epsilon \odelta \EE_{\Zrv_{\sigma}} \Zrv_{\sigma}  - \EE_{\Zrv_{\sigma},\Zrv}\left[ \frac{\orv}{\otaul}( \Prox_{\lossf}(\Zrv_{\sigma}\nupar + \Zrv \nuper - \eps \odelta, \frac{\otaul}{\orv})) \Zrv_{\sigma} \right] 
\end{align}
and hence
\begin{align}
 \nupar  = \frac{ 1}{\EE_{\Zrv_{\sigma}} \Zrv_{\sigma}^2} \left( 
\epsilon \odelta \EE_{\Zrv_{\sigma}} \Zrv_{\sigma}   + \EE_{\Zrv_{\sigma},\Zrv}\left[( \Prox_{\lossf}(\Zrv_{\sigma}\nupar + \Zrv \nuper - \eps \odelta, \frac{\otaul}{\orv})) \Zrv_{\sigma} \right] -  \frac{\otaul}{\orv} 2\lambda \nupar \right).
\end{align}
We can use that $\EE_{\Zrv_{\sigma}} \Zrv_{\sigma} = \sqrt{\frac{2}{\pi}} \left(1 - 2\sigma\right)$ and $\EE_{\Zrv_{\sigma}} \Zrv_{\Sigma}^2 = 1$.

\subsection{Seperable Case}

\begin{theorem}
\label{thm:seperable}
 Assume that $\gamma \geq \gammastar$ and $\lambda = 0$. Furthermore, assume that $\eps = \eps_0/\sqrt{d}$. Let $(\nuper^\star,\nupar^\star, \otaur^\star,  \orv^\star,\odelta^\star,\mu^\star, \kappa^\star,\zeta^\star)$ be the unique solution of
 \begin{equation}
 \begin{split}
 \label{eq:seperable}
  \min_{\substack{\nuper\geq 0, \kappa \\ \nupar, \odelta \geq 0}}\max_{\substack{r,\otaur\geq0}} ~ & \nupar^2 - \kappa \nuper  -\odelta \zeta + \frac{\otaur \kappa}{2} - \frac{\gamma \orv^2}{4(1+\frac{\kappa}{2\otaur}} + 2(1+\frac{ \kappa}{2 \otaur})~\EE_Z \huberloss \left(\frac{Z \sqrt{\gamma} \orv}{2(1+\frac{\kappa}{2 \otaur})}, \frac{\zeta}{2(1+\frac{\kappa}{2 \otaur})} \right) \\
      +& r \sqrt{\EE_{Z,Z_{\sigma}} \left(1+\eps_0\delta - Z_{\sigma} \nupar + Z \nuper\right)_+}
  \end{split}
 \end{equation}
 then asympototiclally as $d/n \to \gamma$, we have that 
 \begin{align}
  \|\thetahat_{\perp} \|_1  &\to \odelta \\
  \| \thetahat^\top \thetanull \|_2 &\to \nupar \\
  \|\thetahat\|_2^2 &\to \nupar^2 + \nuper^2 
 \end{align}
\end{theorem}

 \subsubsection{Proof of Theorem \ref{thm:seperable}}
 \begin{proof}
  We are searching for the max-margin solution which is given by:
  \begin{equation}
   \min_{\theta} \|\theta\|_2^2 ~~\mathrm{sucht~that~forall~}i: \langle \theta, \x_i \rangle - \eps \|\Piper \theta\|_1 \geq 1
  \end{equation}
  Following the same argument as in \cite{Javanmard20b}, we can equivalently write:
  \begin{equation}
  \begin{split}
   &\min_{\theta, \delta}\max_{u: u_i\geq 0, \zeta\geq 0}
   \|\theta\|_2^2 + \frac{1}{n}u^\top \left( 1 + 1 \eps_0 \delta - D_y \Xs \theta\right) + \zeta(\frac{\| \thetaper\|_1}{\sqrt{d}} -\delta) \\
      &\min_{\theta, \delta}\max_{u: u_i\geq 0, \zeta\geq 0}
   \|\theta\|_2^2 + \frac{1}{n}u^\top \left( 1 + 1 \eps_0 \delta - D_y \Xs \Pipar \thetapar - D_y \Xs \Piper \thetaper \right) + \zeta(\frac{\|\thetaper\|_1}{\sqrt{d}} -\delta) \\
   \end{split}
     \end{equation}
    Because $\Xs \Piper$ is independent of $\y$ and $\Xs \Pipar$, we can apply the CGMT: 
    \begin{equation}
  \begin{split}
      &\min_{\theta, \delta}\max_{u: u_i\geq 0, \zeta\geq 0}
   \|\theta\|_2^2 + \frac{1}{n}u^\top \left( 1 + 1 \eps_0 \delta - D_y \Xs \Pipar \thetapar + D_y h \|\thetaper\|_2 \right) + \frac{1}{n}\|u\|_2  g^\top \thetaper + \zeta(\frac{\|\thetaper\|_1}{\sqrt{d}} -\delta) \\
   \end{split}
     \end{equation}
Next, we can solve the optimization over $u$, which gives: 
    \begin{equation}
  \begin{split}
      &\min_{\theta, \delta}\max_{r\geq 0, \zeta\geq 0}
   \|\theta\|_2^2 + \frac{r}{\sqrt{n}}\| \left( 1 + 1 \eps_0 \delta - D_y \Xs \Pipar \thetapar + D_y h \|\thetaper\|_2 \right)_+\|_2 + \frac{r\sqrt{\gamma}}{\sqrt{d}}\|u\|_2  g^\top \thetaper + \zeta(\frac{\|\thetaper\|_1}{\sqrt{d}} -\delta) \\
   \end{split}
     \end{equation}
Next, want to separate $\|\thetaper\|_2$ form the therm in the $(.)_+$ breacket. For this, we can write:
    \begin{equation}
  \begin{split}
      \min_{\nuper\geq 0,\nupar, \delta}\max_{r\geq 0, \zeta\geq 0, \kappa}
   & \nupar^2  +\|\thetaper\|_2^2 +\kappa(\|\thetaper\|_2 - \nuper) + \frac{r}{\sqrt{n}}\| \left( 1 + 1 \eps_0 \delta - D_y \Xs \Pipar \theta_0 \nupar + D_y h \nuper \right)_+\|_2 \\
   + &\frac{r\sqrt{\gamma}}{\sqrt{d}}\|u\|_2  g^\top \thetaper + \zeta(\sqrt{d}\|\Piper \theta\|_1 -\delta) \\
   \end{split}
     \end{equation}
We can now simplify the term in the brackets. For this, note that
\begin{equation}
\begin{split}
 \frac{r}{\sqrt{n}}\| \left( 1 + 1 \eps_0 \delta - D_y \Xs \Pipar \theta_0 \nupar + D_y h \nuper \right)_+\|_2 \to r \sqrt{\EE_{Z,Z_{\sigma}} \left(1+\eps_0\delta - Z_{\sigma} \nupar + Z \nuper\right)_+} =: T 
\end{split}
\end{equation}
Further, we can extend the formula to:
    \begin{equation}
  \begin{split}
      \min_{\nuper\geq 0,\nupar, \delta,\otaur \geq 0}\max_{r\geq 0, \zeta\geq 0, \kappa}
   \nupar^2  + \|\thetaper\|_2^2 +\frac{\kappa}{2\otaur} \|\thetaper\|_2^2 + \frac{\kappa \otaur}{2} -\kappa\nuper + T
   + \frac{r\sqrt{\gamma}}{\sqrt{d}}\|u\|_2  g^\top \thetaper + \zeta(\frac{\|\thetaper\|_1}{\sqrt{d}} -\delta) 
   \end{split}
     \end{equation}
By completion of the squares we get:
    \begin{equation}
  \begin{split}
      \min_{\nuper\geq 0,\nupar, \delta,\otaur \geq 0}\max_{r\geq 0, \zeta\geq 0, \kappa}
   &\nupar^2  + (1+\frac{\kappa}{2\otaur})\|\thetaper + \frac{r \sqrt{\gamma}}{\sqrt{d} 2(1+\frac{\kappa}{2\otaur})} g\|_2^2 - \frac{r^2 \gamma}{ 4 (1+\frac{\kappa}{2 \otaur})} \|g/\sqrt{d}\|_2^2
   \\
   & -\kappa\nuper + T +\zeta(\frac{\|\thetaper\|_1}{\sqrt{d}} - \delta)
   \end{split}
     \end{equation}
In particular, we have that $\|g/\sqrt{d}\|_2^2 \to 1$. It only remains to solve the innter optimization over $\thetaper$. For this, we can write:
\begin{equation}
\begin{split}
 \min_{\thetaper}~&(1+\frac{\kappa}{2\otaur})\|\thetaper + \frac{r \sqrt{\gamma}}{\sqrt{d} 2(1+\frac{\kappa}{2\otaur})} g\|_2^2 +\frac{\|\thetaper\|_1}{\sqrt{d}} \|\thetaper\|_1 \\
 \overset{\tilde{\thetaper} = \frac{\thetaper}{\sqrt{d}}}= \min_{\tilde{\thetaper}} &\frac{1}{d} (1+\frac{\kappa}{2\otaur})\| \tilde{\thetaper} +\frac{r \sqrt{\gamma}}{2(1+\frac{\kappa}{2\otaur})} g \| + \zeta \frac{\|\thetaper\|_1}{d}
 \\ = &\frac{1}{d} \sum_{i=2}^d  \min_{\tilde{\thetaper}_i}~ (1+\frac{\kappa}{2\otaur})(\tilde{\thetaper}_i +\frac{r \sqrt{\gamma}}{ 2(1+\frac{\kappa}{2\otaur})} g_i)^2 +  \zeta \abs{\tilde{\thetaper}_i}
   \\ = &\frac{1}{d} 2(1+\frac{\kappa}{2\otaur}) \sum_{i=2}^d  \min_{\tilde{\thetaper}_i}~ \frac{1}{2}(\tilde{\thetaper}_i +\frac{r \sqrt{\gamma}}{ 2(1+\frac{\kappa}{2\otaur})} g_i)^2 + \frac{\zeta}{2(1+\frac{\kappa}{2\otaur})} \abs{\tilde{\thetaper}_i}
    \\ = &\frac{1}{d} 2(1+\frac{\kappa}{2\otaur}) \sum_{i=2}^d  \huberloss(-\frac{r \sqrt{\gamma}}{ 2(1+\frac{\kappa}{2\otaur})} g_i, \frac{\zeta}{2(1+\frac{\kappa}{2\otaur})})
\\ \to  & 2(1+\frac{\kappa}{2\otaur}) \EE_Z ~\huberloss \left(\frac{r \sqrt{\gamma}}{ 2(1+\frac{\kappa}{2\otaur})} Z, \frac{\zeta}{2(1+\frac{\kappa}{2\otaur})}\right)
 \end{split}
\end{equation}
where $\huberloss$ is the Huber loss, which is given by $\huberloss(x,y) = \left\{ \begin{matrix} 0.5 x^2 ~~\abs{x} \leq y \\ y (\abs{x} - 0.5 y)                                                                                       \end{matrix} \right.$

\end{proof}

\subsubsection{System of equations}

The goal is again to solve the optimization problem by formulation a system of equations. First, note that $\EE_Z (b+aZ)_+^2 = (b^2+a^2)/2(1+\erf(\frac{b}{\sqrt{2}a})) + \frac{a b}{\sqrt{2 \pi}} \exp(-b^2/(2 a^2))$. Hence, we cna write
\begin{equation}
 \sqrt{\EE_{Z,Z_{\sigma}} \left(1+\eps_0\delta - Z_{\sigma} \nupar + Z \nuper\right)_+} = \sqrt{\EE_{Z_{\sigma}} (b^2+a^2)/2(1+\erf(\frac{b}{\sqrt{2}a})) + \frac{a b}{\sqrt{2 \pi}} \exp(-b^2/(2 a^2))} =: \sqrt{T}
\end{equation}
with $a = \nuper$ and $b = 1+\eps_0\delta - Z_{\sigma} \nupar$. We use the following shorthand notation: Let $H = \EE_Z \huberloss \left(\frac{Z \sqrt{\gamma} \orv}{2(1+\frac{\kappa}{2 \otaur})}, \frac{\zeta}{2(1+\frac{\kappa}{2 \otaur})} \right)  $ be the expected huber loss and for the derivatives let $H_x$ denotes the derivative with respect to the first input of the Huber loss and $H_y$ of the second. Furthermore, we denote with $T_{\nuper}$ the derivative with respect to $\nuper$ and similarily for the other variables. In particular, we have
\begin{align}
 T_{\nupar} &= - \EE_{Z_{\sigma}} Z_{\sigma} \left(\frac{2a}{\sqrt(2\pi)} \exp(-b^2/(2 a^2))  + b \erf(b/(\sqrt(2)a))+b \right)\\
 T_{\nuper} &= \EE_{Z_{\sigma}} 2 a (1+\erf(\frac{b}{\sqrt{2} a})) \\
 T_{\delta} &= \eps_0 \EE_{Z_{\sigma}} \frac{2a}{\sqrt(2\pi)} \exp(-b^2/(2 a^2))  + b \erf(b/(\sqrt(2)a))+b
\end{align}

Define $s = (1+\frac{\kappa}{2\otaur})$. Recall that the optimization objective is 
\begin{equation}
 C = \nupar^2 -\kappa \nuper - \delta \zeta - \frac{\gamma r^2}{4 s} +2s H + r \sqrt{T} + \frac{\otaur \kappa}{2}
\end{equation}
The goal is now to find a system of fixed point equations from $\nabla C = 0$.
First note that:
\begin{align}
 H_{r} &= 2 s H_x \frac{\sqrt{\gamma}}{2s} = H_x \sqrt{\gamma}\\
 H_{\kappa} &= 2 \frac{1}{2 \otaur} H - 2 s H_x \frac{\sqrt{\gamma} r}{2s^2}\frac{1}{2 \otaur} - 2s H_y \frac{\zeta}{2s^2}\frac{1}{2\otaur} \\
 &=  \frac{1}{\otaur} H - H_x \frac{\sqrt{\gamma} r}{s} \frac{1}{2\otaur}  -  H_y \frac{\zeta}{s} \frac{1}{2\otaur} \\
 H_{\otaur} &= -\frac{\kappa}{\otaur^2} H + H_x \frac{\sqrt{\gamma} r}{s} \frac{\kappa}{2\otaur^2}  +  H_y \frac{\zeta}{s} \frac{\kappa}{2\otaur^2} \\
  H_{\zeta} &= 2 s H_y \frac{1}{2s} = H_y \\
\end{align}
We can now solve: 
\begin{align}
 \frac{\partial}{\partial \nupar} C &= 2\nupar + \frac{1}{2 \sqrt{T}} r T_{\nupar} \\
  \frac{\partial}{\partial \delta} C &= - \zeta +\frac{1}{2 \sqrt{T}} r T_{\delta} \\
\frac{\partial}{\partial \nuper} C &= - \kappa +\frac{1}{2 \sqrt{T}} r T_{\nuper} \\
\frac{\partial}{\partial \zeta} C &= - \delta  + H_{y} \\
\frac{\partial}{\partial \kappa} C &= - \nuper  + H_{\kappa} + \frac{\gamma r^2}{4 s^2} \frac{1}{2\otaur} + \frac{\otaur}{2} \\
\frac{\partial}{\partial \otaur} C &=  H_{\otaur} - \frac{\gamma r^2}{4 s^2} \frac{\kappa}{2\otaur^2} + \frac{\kappa}{2} \\
\frac{\partial}{\partial \orv} C &=  \sqrt{T} + H_{r} - \frac{\gamma r}{2 s}  \\
\end{align}

Hence, we have
\begin{align}
 \nupar &= -\frac{1}{4 \sqrt{T}} r T_{\nupar}\\
  \kappa &= \frac{1}{2 \sqrt{T}} r T_{\nuper}\\
 \zeta &= \frac{1}{2 \sqrt{T}} r T_{\delta}\\
 \nuper &= H_{\kappa} + \frac{\gamma r^2}{2 s^3} \frac{1}{2\otaur}+ \frac{\otaur}{2} \\
 \delta &= H_y\\
\orv &= (\sqrt{T} +H_r )\frac{2 s^2}{\gamma}\\
\otaur^2 &= -2 H + H_x \frac{\sqrt{\gamma} r}{s} + H_y \frac{\zeta}{s}    -\frac{\gamma r^2}{2 s^3}  \\
\end{align}

\subsection{Implementation details}

\subsubsection{Implementation of theoretical curves}
\label{sec:logregopt}

How you solve the optimization problem.
