# Supplementary material for: Interpolation can hurt robust generalization even when there is no noise
Source: arXiv:2108.02883 source file (2021-12-16)
Supplement: Supplementary file 6 [file logreg_theory.tex]

\section{Details on Theorem~\ref{theo:logreg}}
\label{sec:logregtheory}

In this section we give a formal statement for Theorem \ref{theo:logreg}. The results are based on the Convex Gaussian Minimax Theorem (CGMT)\cite{Gordon88,Thrampoulidis15}.
The results presented in this section have similarities with the ones in \cite{Javanmard20b}, however, we study the discriminative data model with features drawn from a single Gaussian and  $1$-sparse ground truth. In contrast, in the paper \cite{Javanmard20b}, the authors study a generative data model with features drawn from two Gaussians. 
Furthermore, while not for adversarial training, several papers have already studied standard logistic regression for isotropic Gaussian features in high dimensions \cite{Salehi19,Sur19}.

An immediate consequence of the proof of Lemma \ref{lm:logregrisk} is that the adversarial loss from Equation~\eqref{eq:ridgeloss}  writes as
\begin{equation}
\label{eq:logregrisk}
 \empriskrob(\theta) = \frac{1}{n} \sum_{i=1}^n \losstrain(y_i \langle\theta,\x_i\rangle - \eps\|\Piper \thetahat\|_1) + \lambda \|\theta\|_2^2.
\end{equation}
Note that the equation holds for consistent $\ell_{\infty}$ perturbations with logistic loss ${\losstrain(x) = \log(1+\exp(-x))}$ and $1$-sparse ground truth.

Let  $\Moreau_f(\x,t) = \min_{y} \frac{1}{2t}(x-y)^2 + f(y)$ be the Moreau envelope and let $\Zpar,\Zperp$ be two independent standard normal distributed random variables. We can now state Theorem~\ref{thm:nonseperable} which describes the asymptotic risk of $\thetaepslambda$, for $\lambda > 0$, and for
% \rh{Throughout this appendix, is $\thetahat$ equal to $\thetaepslambda$? If yes let's use the latter - we need to be consistent with the notation used in the main body.}
the asymptotic regime where $d,n \to \infty$. The proof of the theorem can be found in \suppmat{}~\ref{sec:proofnonseperable}.

\begin{theorem}
\label{thm:nonseperable}
Assume that the we have \iid random features $\x_i$ drawn form an isotropic Gaussian with noiseless observations $\y_i = \sgn(\langle x_i, \thetastar\rangle)$ and ground truth $\thetastar = (1,0,\hdots,0)^\top$. Further, assume that $\lambda >0$ and $\eps = \eps_0/\sqrt{d}$, where $\eps_0$ is a numerical constant. Let $(\nuper^\star,\nupar^\star,  \orv^\star,\odelta^\star,\mu^\star, \tau^\star )$ be the unique solution of
 \begin{equation}
 \begin{split}
 \label{eq:nonseperable}
  \min_{\substack{\nuper\geq 0, \tau\geq 0, \\ \nupar, \odelta \geq 0}}\max_{\substack{r\geq 0, \\ \mu\geq 0}} ~ &\EE_{\Zpar,\Zperp}\left[ \Moreau_{\lossf}(\abs{\Zpar} \nupar + \Zperp \nuper - \eps_0 \odelta, \frac{\tau}{\orv})\right]  - \odelta \mu +\frac{\orv \tau}{2} + \lambda(\nuper^2 +\nupar^2) \\
%       -\odelta&\EE_{\Zperp}\left[ \Moreau_{\vert.\vert}(\orv \sqrt{\gamma} \Zperp, \frac{\otaur\odelta}{\nuper})\right]
      -&\nuper \sqrt{\left[ (\mu^2+\gamma\orv^2) -  (\mu^2+\gamma\orv^2) \erf(\mu/(\sqrt{\gamma}\orv\sqrt{2})) - \sqrt{\frac{2}{\pi}} \sqrt{\gamma}\orv\mu \exp(-\mu^2/(\gamma \orv^2 2)) \right]} .
      \end{split}
 \end{equation}
 Then, for $\lambda >0$ the estimator $\thetaepslambda$ from Equation \eqref{eq:ridgeloss} with logistic loss and consistent $\ell_{\infty}$ attacks satisfies asymptotically as $d,n\to\infty$, $d/n \to \gamma$ 
 \begin{align}
 \label{eq:solnonsep}
  \frac{1}{\sqrt{d}} \|\Piper \thetaepslambda \|_1  \to \odelta ~~\mathrm{and}~~
   \langle \thetaeps,  \thetanull \rangle  \to \nupar ~~\mathrm{and}~~
  \|\thetaepslambda \|_2^2 \to \nupar^2 + \nuper^2.
 \end{align}
  The convergences hold true in probability. 

\end{theorem}

 For $\lambda >0$, the loss in Equation~\eqref{eq:logregrisk} has a unique minimizer. In contrast, for $\lambda = 0$ the minimizer of the loss in Equation \eqref{eq:logregrisk} is not unique since the observations are noiseless and the adversarial attacks are consistent. 
As discussed in Section \ref{sec:logreg}, we study instead the penalized max-margin solution from Equation \eqref{eq:maxmarginAE}. The asymptotic behavior of the corresponding solution is characterized in Theorem \ref{thm:seperable} with proof in \suppmat{}~\ref{sec:proofseperable}. 

\begin{theorem}
\label{thm:seperable}
 Assume that the we have \iid random features $\x_i$ drawn form an isotropic Gaussian with noiseless observations $\y_i = \sgn(\langle x_i, \thetastar\rangle)$ and $\thetastar = (1,0,\cdots,0)^\top$ as describes in Section \ref{sec:logreg}. Further, assume that $\eps = \eps_0/\sqrt{d}$. Let $(\nuper^\star,\nupar^\star,   \orv^\star,\odelta^\star, \zeta^\star,\kappa^\star)$ be the unique solution of
%  \rh{I don't understand the $( \cdot )_+$ here - is the the relu function?  Pls define. Also, is the expectation squared or is expectation over the squared function? I assume the latter, but better to be clear with the notation here.}
 \begin{equation}
 \begin{split}
 \label{eq:seperable}
  \min_{\substack{\nuper\geq 0, \\  \odelta \geq 0,\kappa, \nupar}}\max_{\substack{\zeta, r \geq 0}} ~ & \nupar^2 - \kappa \nuper^2  -\odelta \zeta - \frac{\gamma \orv^2}{4(1+\kappa} +  r \sqrt{\EE_{\Zpar, \Zperp} \left[ \max\left(0,1+\eps_0\delta - \abs{\Zpar} \nupar + \Zperp \nuper\right)^2 \right]} \\+& \frac{1}{2(1+\kappa)} \left(\frac{\gamma \orv^2+\zeta^2}{2}\erf\left(\frac{\zeta}{\sqrt{2} \sqrt{\gamma} \orv}\right) - \frac{\zeta^2}{2} + \frac{\sqrt{\gamma} \orv \zeta}{\sqrt{2 \pi}} \exp\left(- \frac{\zeta^2}{2 \gamma \orv^2} \right) \right).
  \end{split}
 \end{equation}
 Then, the estimator $\thetaeps$ from Equation \eqref{eq:maxmarginAE} with logistic loss and consistent $\ell_{\infty}$ attacks satisfies asymptotically as $d,n\to\infty$, $d/n \to \gamma$ 
 \begin{align}
 \label{eq:solsep}
  \frac{1}{\sqrt{d}} \|\Piper \thetaeps \|_1  \to \odelta ~~\mathrm{and}~~
  \langle \thetaeps,  \thetanull \rangle \to \nupar ~~\mathrm{and}~~
  \|\thetaeps \|_2^2 \to \nupar^2 + \nuper^2.
 \end{align}
  The convergences hold true in probability. 
\end{theorem}

\begin{remark}
 Theorem \ref{theo:logreg} is obtained form Theorem \ref{thm:nonseperable},\ref{thm:seperable} when inserting the expression from Equation \eqref{eq:solnonsep},\eqref{eq:solsep} into the expression of the risk in Lemma \ref{lm:logregrisk}. 
\end{remark}

%%%
\subsection{Solving the optimization problems}
To obtain concrete predictions from Theorems \ref{thm:nonseperable} and \ref{thm:seperable} we need to solve the corresponding optimization problems. 
% We next explain how to solve those optimization problems numerically.  
%We now give some additional details on how to solve the optimization problems in Theorem \ref{thm:nonseperable},\ref{thm:seperable}.
Using the fact that the objective is concave in $r, \mu$ respectively $r, \otaur$ and convex in all other variables, we 
find the unique solution by solving the systems of equations stated in 
Corollary~\ref{cor:nonseperable},\ref{cor:seperable} presented below --- assuming that the solution is not obtained on the boundary. For numerical predictions, we solve the systems of equations using a least squares solver in \emph{MATLAB} where we approximated the expectations using a standard numerical integrator.
 
 \paragraph{Regularization $\lambda >0$:}
 We make use of the following well known facts on the derivative of the Moreau envelope (e.g. see~\cite{Jourani14}):
\begin{align*}
\frac{\partial \Moreau_{f}(x,t)}{\partial x} = \frac{1}{t}(x - \Prox_f(x,t))
~~\mathrm{and}~~
\frac{\partial \Moreau_{f}(x,t)}{\partial t} = -\frac{1}{2t^2}(x - \Prox_f(x,t))^2
\end{align*}
where $\Prox_f(x,\mu)$ is the proximal operator
\begin{equation*}
 \Prox_f(x,\mu) = \arg\min_{t} f(t) + \frac{1}{2\mu}(t-x)^2.
\end{equation*}
Let $\EMoreau = \EE_{\Zpar,\Zperp}\left[ \Moreau_{\lossf}(\Zpar\nupar + \Zperp \nuper - \eps \odelta, \frac{\tau}{\orv})\right]$ and denote with ${\EMoreau_{\nupar} = \EE_{\Zpar,\Zperp}\left[ \frac{\partial_x\Moreau_{\lossf}}{\partial x}(\Zpar\nupar + \Zperp \nuper - \eps \odelta, \frac{\tau}{\orv}) \frac{\partial (\Zpar\nupar + \Zperp \nuper - \eps \odelta)}{\partial \nuper}\right]}$ the derivative of the expected Moreau envelope with respect to $\nupar$ and similar for the other variables.

Further, define ${\expterms =  (\mu^2+\gamma\orv^2) -  (\mu^2+\gamma\orv^2) \erf(\mu/(\sqrt{\gamma}\orv\sqrt{2})) - \sqrt{\frac{2}{\pi}} \sqrt{\gamma}\orv\mu \exp(-\mu^2/(\gamma \orv^2 2))}$ and denote with $ g_{\mu}$ respectively $g_{\orv}$ the corresponding partial derivatives. This allows us to express the optimization objective form Theorem \ref{thm:nonseperable} as
\begin{equation*}
  C =   \EMoreau - \nuper \sqrt{g(\mu,\orv)} - \odelta \mu 
    +\frac{\orv \tau}{2} + \lambda(\nuper^2 +\nupar^2).
\end{equation*}
 Since the problem is concave in $r,\mu$ and convex in the other variables,
  we can equivalently solve the the system of equations $\nabla C = 0$, which gives us the following corollary.
\begin{cor}
 \label{cor:nonseperable}
 Assume that the solution of Equation \eqref{eq:nonseperable} form Theorem \ref{thm:nonseperable} is not obtained on the boundary. Then, the solution  satisfies the following system of Equations. 
 \begin{align*}
0 &= \frac{\partial }{\partial \nupar} C = \EMoreau_{\nupar} + 2\lambda \nupar \\
0 &= \frac{\partial }{\partial \nuper} C = \EMoreau_{\nuper} + 2\lambda \nuper -\sqrt{g}\\
0 &= \frac{\partial }{\partial \orv} C = \EMoreau_{\orv} -\frac{\nuper}{2\sqrt{g}} g_{\orv} + \frac{\tau}{2} \\
0 &= \frac{\partial }{\partial \odelta} C = \EMoreau_{\odelta} - \mu \\
0 &= \frac{\partial }{\partial \mu} C =-\frac{\nuper}{2 \sqrt{g}} g_{\mu} - \delta  \\
0 &= \frac{\partial }{\partial \tau} C = \EMoreau_{\tau} + \frac{r}{2}\\
\end{align*}
\end{cor}

\subsection{Interpolation $\lambda = 0$:}
 
 Similarly, we can also reformulate the optimization problem in Theorem \ref{thm:seperable}. Again, for brevity of notation, let $T = \EE_{Z,Z_{\sigma}} \left(1+\eps_0\delta - Z_{\sigma} \nupar + Z \nuper\right)^2_+$ and ${H =  \left(\frac{\gamma \orv^2+\zeta^2}{2}\erf\left(\frac{\zeta}{\sqrt{2} \sqrt{\gamma} \orv}\right) - \frac{\zeta^2}{2} + \frac{\sqrt{\gamma} \orv \zeta}{\sqrt{2 \pi}} \exp\left(- \frac{\zeta^2}{2 \gamma \orv^2} \right) \right)  }$. Further, denote with $T_{\nuper}$ the derivative with respect to the corresponding variable and similarly for $H_{r}$. As a result, we can write the optimization objective from Theorem \ref{thm:seperable} as 
 \begin{equation*}
 C = \nupar^2 -\kappa \nuper^2 - \delta \zeta - \frac{\gamma r^2}{4 s} +2s H + r \sqrt{T} + \frac{\otaur \kappa}{2}.
 \end{equation*}
Since the solution of the optimization problem satisfies again $\nabla C = 0$, we analogously obtain the following corollary. 
 \begin{cor}
 \label{cor:seperable}
 Assume that the solution of Equation \eqref{eq:seperable} form Theorem \ref{thm:seperable} is not obtained on the boundary. Then, the solution  satisfies the following system of Equations. 
 \begin{align*}
 0 &= \frac{\partial}{\partial \nupar} C = 2\nupar + \frac{1}{2 \sqrt{T}} r T_{\nupar} \\
 0 &= \frac{\partial}{\partial \nuper} C = - 2\kappa \nuper  +\frac{1}{2 \sqrt{T}} r T_{\nuper} \\
0 &=\frac{\partial}{\partial \orv} C =  \sqrt{T} + H_{r} - \frac{\gamma r}{2 (1+\kappa)}  \\
  0 &= \frac{\partial}{\partial \delta} C = - \zeta +\frac{1}{2 \sqrt{T}} r T_{\delta} \\
  0 &= \frac{\partial}{\partial \zeta} C = - \delta  + H_{y} \\
0 &= \frac{\partial}{\partial \kappa} C = - \nuper^2  + H_{\kappa} + \frac{\gamma r^2}{4 (1+\kappa)^2}  
\end{align*}

\end{cor}

%  The goal is again to solve the optimization problem by formulation a system of equations. First, note that $\EE_Z (b+aZ)_+^2 = (b^2+a^2)/2(1+\erf(\frac{b}{\sqrt{2}a})) + \frac{a b}{\sqrt{2 \pi}} \exp(-b^2/(2 a^2))$. Hence, we cna write
% \begin{equation}
%  \sqrt{\EE_{Z,Z_{\sigma}} \left(1+\eps_0\delta - Z_{\sigma} \nupar + Z \nuper\right)_+} = \sqrt{\EE_{Z_{\sigma}} (b^2+a^2)/2(1+\erf(\frac{b}{\sqrt{2}a})) + \frac{a b}{\sqrt{2 \pi}} \exp(-b^2/(2 a^2))} =: \sqrt{T}
% \end{equation}
% with $a = \nuper$ and $b = 1+\eps_0\delta - Z_{\sigma} \nupar$. We use the following shorthand notation: Let $H = \EE_Z \huberloss \left(\frac{Z \sqrt{\gamma} \orv}{2(1+\kappa)}, \frac{\zeta}{2(1+\kappa)} \right)  $ be the expected huber loss and for the derivatives let $H_x$ denotes the derivative with respect to the first input of the Huber loss and $H_y$ of the second. Furthermore, we denote with $T_{\nuper}$ the derivative with respect to $\nuper$ and similarily for the other variables. In particular, we have 
%  

\subsection{Label noise}

While our results assume noiseless observations $y_i = \sgn(\langle x_i, \thetastar\rangle)$, Theorem~\ref{thm:nonseperable},\ref{thm:seperable} can be extended to the case where additional label noise is added to the observations. That is, it can be extended to the case where $y_i = \sgn(\langle x_i, \thetastar\rangle) \xi$ with $\prob(\xi = 1) = 1- \sigma$ and $\prob(\xi = -1) = \sigma$. Note that the only modification need for both theorems is to replace $\abs{\Zpar}$ with $\xi \abs{\Zpar}$. 

However, as discussed in Section \ref{sec:logregnoise}, label noise in the train data may prevent interpolation even when $\lambda=0$ and hence Equation \eqref{eq:logregrisk} may also have a unique bounded solution for $\lambda = 0$. In fact, we note that the asymptotic threshold $\gamma^\star$ such that the train loss does not vanish with high probability for all $\gamma < \gamma^\star$ and vanishes with high probability for all $\gamma \geq \gamma^\star$ as $d/n \to \gamma$ can be found when solving a low dimensional scalar optimization problem similar to Theorem 6.1 \cite{Javanmard20b}.

% 
% thus the noise might prevent the unregulated estimator from achieving a vanishing train loss. This is also discussed in \suppmat{} \ref{sec:logregnoise}. 

\subsection{Proof of Theorem \ref{thm:nonseperable}}
 \label{sec:proofnonseperable}
The proof is similar to the proof of Theorem 6.4 \cite{Javanmard20b}. Denote with $\Xs \in \RR^{n \times d}$ the input data matrx and with $y \in \RR^n$ the vector containing the observations.
Recall that the estimator $\thetahat$ is given by
\begin{align}
 \thetahat &= \arg\min_{\theta} \frac{1}{n} \sum_{i = 1}^{n} \lossf(\y_i \langle x_i, \theta \rangle - \eps  \|\Piper \theta\|_1) + \lambda \|\theta\|_2^2 \nonumber \\
 &= \arg\min_{\theta} \frac{1}{n} \sum_{i = 1}^{n} \lossf( v_i - \eps  \|\Piper \theta\|_1) + \lambda \|\theta\|_2^2 ~~\mathrm{such~that~} v  = D_y \Xs \theta, \label{eq:thmnonsepridge}
\end{align}
where $\lossf(x) = \log(1+\exp(-x))$ is the logistic loss, $\Xs \in \RR^{n\times d}$ is the data matrix and $D_y$ the diagonal matrix with entries $(\Dy)_{i,i} = \y_i$. We can then introduce the Lagrange multiplier $u$  to obtain:
\begin{equation*}
 \min_{\theta,v} \max_{u} ~\frac{1}{n} \sum_{i=1}^{n} \lossf(v_i - \eps \|\Piper \theta\|_1) + \frac{1}{n} u^\top \Dy \Xs \theta - \frac{1}{n} u^\top v+ \lambda \|\theta\|_2^2.
\end{equation*}
% where 
% Define $\Xs \Pipar = \Xs \Pi_{\parallel}$ 
% 
% \rh{Shouldn't it be $\Pi_{\parallel}\X$ instead? If not, I don't understand what's going on. }
% 
% and $\Xs \Piper = \Xs \Pi_{\perp}$, which allows us to write
% 
% \rh{Every few lines you introduce a new variable or notation - this makes it extremely difficult to verify correctness and follow the proof. Is this really necessary? $\Xs \Piper$ is only used once, so it seems unnecessary! We need to simplify the notation to make this readable.}
Furthermore, we can separate $\Xs = \Xs \Piper + \Xs\Pipar$, which gives us:
\begin{align*}
 \min_{\theta,v} \max_{u} ~ \frac{1}{n} \sum_{i=1}^{n} \lossf(v_i - \eps \|\Piper \theta\|_1) + \frac{1}{n} u^\top \Dy \Xs \Pipar \theta 
 +\frac{1}{n} u^\top \Dy \Xs \Piper \theta - \frac{1}{n} u^\top v + \lambda \|\theta\|_2^2.
\end{align*}

\paragraph{Convex Gaussian Minimax Theorem}
We can now make use of the CGMT, which states that 
\begin{equation}
\label{eq:primalcgmt}
 \min_{\theta \in U_{\theta}} \max_{u \in U_{u}} u^\top \Xs \theta + \psi(u,\theta),
\end{equation}
with $\psi$ convex in $\theta$ and concave in $u$ has asymptotically point wise the same solution when $d,n\to\infty$, $d/n \to \gamma$ as 
\begin{equation}
\label{eq:auxiliarycgmt}
 \min_{\theta \in U_{\theta}} \max_{u \in U_{u}} \|u\|_2 g^\top \theta + u^\top h \|\theta\|_2 + \psi(u,\theta),
\end{equation}
with $g \in \RR^n$, $u\in \RR^d$ random vectors with \iid{} standard normal distributed entries. Here, the sets $U_{\theta}$ and $U_u$ are compact. As commonly referred to in the literature, we call Equation \eqref{eq:primalsep} the primal optimization problem and Equation \eqref{eq:auxiliarycgmt} the auxiliary optimization problem. 
We refer to \cite{Thrampoulidis15} for the precise statement.

% \rh{If you use the statement, can't you just state it here? Saying see ``for the precise statement'' is a bit vague.}

Since $\Xs \Piper$ is independent of the observations $\y$ and of $\Xs \Pipar$, and because Equation~\eqref{eq:thmnonsepridge} has a unique bounded solution as $\lambda >0$, we can apply the CGMT, which gives:

% forwardly verify that all the assumptions for the CGMT hold. 

% \rh{Unclear because the CGMT is not stated here..}

% Hence, we can write
\begin{align*}
 \min_{\theta,v} \max_{u} ~ &\frac{1}{n} \sum_{i=1}^{n} \lossf(v_i - \eps \|\Piper \theta\|_1) + \frac{1}{n} u^\top \Dy \Xs \Pipar \theta +\frac{1}{n} \|u^\top \Dy\|_2 g^\top \Piper \theta \\ +&\frac{1}{n} u^\top \Dy h \| \Piper \theta \|_2  - \frac{1}{n} u^\top v + \lambda \|\theta\|_2^2,
\end{align*}
where $g\in\RR^d$ and $h\in \RR^n$ are vectors with \iid{} standard normal distributed entries. 
\paragraph{Scalarization of the optimization problem} We now aim to simplify the optimization problem. 
In a first step, we maximize over $u$. For this, define $\orv =  \|u\|_2/\sqrt{n}$, which allows us to equivalently write:
 \begin{equation*}
 \min_{\theta,v} \max_{\orv \geq 0} ~~ \frac{1}{n} \sum_{i=1}^{n} \lossf(v_i - \eps \|\Piper \theta\|_1) + \frac{r}{\sqrt{n}} \|\Dy \Xs \Pipar \theta  + \Dy h \| \Piper \theta \|_2  -  v \|_2 +\frac{1}{\sqrt{n}} \orv g^\top \Piper \theta + \lambda \|\theta\|_2^2,
\end{equation*}
where we have used the fact that $\|u^\top \Dy\|_2 = \|u\|_2$. Next, we note that because the problem is convex in $\orv$ and concave in $\theta,v$, we can swap maximization with minimization. In order to proceed, we want to separate $\Piper \theta$ form the loss  $\lossf(v,\Piper \theta) := \frac{1}{n} \sum_{i=1}^{n} \lossf(v_i - \eps \|\Piper \theta\|_1)$. We can write $\lossf(v,\Piper \theta)$ in terms of its conjugate with respect to $\Piper \theta$: 
\begin{equation*}
 \lossf(v,\Piper \theta) = \sup_{w} \frac{1}{\sqrt{d}}w^\top  \Piper \theta - \conjlossf(v,w),
\end{equation*}
where $\conjlossf$ is the conjugate of $\lossf$. In particular, we can use Lemma A.2 in the paper \cite{Javanmard20b} which shows that
\begin{equation*}
 \conjlossf(v,w) = \sup_{\odelta \geq 0} \frac{\sqrt{d}}{\sqrt{d}}\odelta \|w\|_{\infty} - \frac{1}{n} \sum_{i=1}^n \lossf(v_i - \sqrt{d}\eps \odelta) = \sup_{\odelta \geq 0} \odelta \|w\|_{\infty} - \frac{1}{n} \sum_{i=1}^n \lossf(v_i - \eps_0 \odelta).
\end{equation*}
Interchanging the order of maximization over $w$ and minimization over $\delta$, we get
\begin{align}
\label{eq:delta}
 \max_{\substack{r\geq 0}} \min_{\substack{\theta,v,\\ \odelta\geq0}} ~~\frac{1}{n} &\sum_{i=1}^n \lossf(v_i - \eps_0 \odelta)  + \frac{r}{\sqrt{n}} \left\|\Dy \Xs \Pipar \theta + \Dy h \| \Piper \theta \|_2  -  v \right\|_2 + \lambda \|\theta\|_2^2 \\  +& \max_w\left[ \frac{1}{\sqrt{d}}w^\top \Piper \theta - \odelta \|w\|_{\infty}  + \frac{1}{\sqrt{n}} \orv g^\top \Piper \theta \right]  \nonumber
\end{align}
where we used again the fact that we can interchange the order maximization and minimization. 
Next, we simplify the optimization over $\theta$. Write $\Pipar \theta = \Pipar 1 \nupar$ where $\nupar \in \RR$ and let $\nuper = \|\Piper \theta\|_2$. We can simplify
\begin{align}
\label{eq:nuperpar}
 \max_{\substack{r\geq 0}} \min_{\substack{\nuper \geq 0,\\ \odelta\geq0, \\ \nupar, v}} ~~&\frac{1}{n} \sum_{i=1}^n \lossf(v_i - \eps_0 \odelta) 
  + \frac{r}{\sqrt{n}} \|\Dy \Xs \Pipar 1 \nupar  + \Dy h \nuper  -  v \|_2  + \lambda (\nupar^2 +\nuper^2)\\ 
  +& \max_w  \left[- \frac{1}{\sqrt{d}}\nuper \| \Piper(w - \sqrt{\gamma} \orv g)\|_2  -\odelta \|w\|_{\infty} \right] \nonumber
\end{align}
In order to obtain a low dimensional scalar optimization problem, we still need to scalarize the optimization over $w$ and $v$. For this, we replace the term $ \|\Dy \Xs \Pipar 1 \nupar  + \Dy h \nuper  -  v \|_2 $ with its square, which is achieved by using the following identity $\min_{\tau\geq0} \frac{x^2}{2\tau} + \frac{\tau}{2} = x$. 
Hence, 
\begin{align*}
\max_{\substack{r\geq 0}} \min_{\substack{\nuper \geq 0, \tau \geq 0\\ \odelta\geq0, \\ \nupar, v}}~~ &\frac{1}{n} \sum_{i=1}^n \lossf(v_i - \eps_0 \odelta) 
+\frac{\orv}{2\tau n} \|\Dy \Xs \Pipar 1 \nupar   + \Dy h \nuper  -  v \|_2^2+ \frac{\tau \orv}{2}  + \lambda (\nupar^2 +\nuper^2)
  \\
  +& \max_w  \left[- \frac{1}{\sqrt{d}}\nuper \| \Piper(w - \sqrt{\gamma} \orv g)\|_2  -\odelta \|w\|_{\infty} \right]
\end{align*}
interchanging again the order of maximization and minimization, we can now separately solve the following two inner optimization problems:
\begin{align*}
 &\max_{w}~ - \nuper\frac{1}{d}\| \Piper(w - \sqrt{\gamma} \orv g)\|_2  -\odelta \|w\|_{\infty} \\
 &\min_{v}~ \frac{\orv}{2\tau n} \|\Dy \Xs \Pipar 1 \nupar +  \Dy h \nuper  -  v \|_2^2 +  \sum_{i=1}^n \lossf(v_i - \eps_0 \odelta) 
\end{align*}
\paragraph{First term}
 Let $\SoftT_t(x) = \left\{\begin{matrix} 0 & \abs{x} \leq t \\ \sgn(x)(\abs{x}-t) &\mathrm{else}                                                         
\end{matrix}\right. $ be the soft threshold function. We have
\begin{align*}
 &\max_{w}~ -\nuper \frac{1}{\sqrt{d}}\| \Piper(w - \sqrt{\gamma} \orv g)\|_2  -\odelta \|w\|_{\infty} \\
 = - &\min_{w}~  \nuper\frac{1}{\sqrt{d}}\| \Piper(w - \sqrt{\gamma} \orv g)\|_2  -\odelta \|w\|_{\infty} \\ 
 \overset{\mu = \|w\|_{\infty}}{=} -&\min_{\mu \geq0} \nuper~ \sqrt{ \frac{1}{d} \sum_{i=2}^d \left(\SoftT_{\mu}\left(\sqrt{\gamma} \orv g_i\right)\right)^2} +\odelta \mu \\
  \overset{\mathrm{LLN~as~} d\to \infty}{\to} -&\min_{\mu \geq0} \nuper~ \sqrt{\EE_Z \left(\SoftT_{\mu}\left(\sqrt{\gamma} \orv Z \right)\right)^2} +\odelta \mu,
\end{align*}
where we used in the third line that the ground truth $\thetastar$ is $1$-sparse and in the last line that the expectation exists. Finally, we can further simplify
\begin{align*}
 \EE_Z \left(\SoftT_{\mu}\left(\sqrt{\gamma} \orv Z \right)\right)^2 &= \gamma r^2 \EE_Z \left(\SoftT_{\mu/(\sqrt{\gamma}r)}\left( Z \right)\right)^2 \\
 &= \gamma r^2 \EE_Z (Z- \mu/(\sqrt{\gamma} r))^2 - \EE_Z \indicator_{\abs{Z} \leq \mu/(\sqrt{\gamma} r)} (Z- \mu/(\sqrt{\gamma} r))^2 \\
 &=  (\mu^2+ \gamma r^2)\left(1 -  \erf(\mu/(\sqrt{2\gamma} r)) \right)- \sqrt{\gamma} r \mu \sqrt{\frac{2}{\pi}}  \exp(-\mu/(2 \gamma r^2 )).
\end{align*}
Hence, we can conclude the first term.

\paragraph{Second term}
For the second term we also aim to apply the law of large numbers. We have
\begin{align*}
  &\min_{v}~ \frac{\orv}{2\tau n} \|\Dy \Xs \Pipar 1 \nupar  + \Dy h \nuper  -  v \|_2^2 +  \frac{1}{n}\sum_{i=1}^n \lossf(v_i - \eps_0 \odelta) \\
  \overset{\tildev = v - \eps\odelta}{=} &\min_{\tildev}~  \frac{\orv}{2\tau n} \|\Dy \Xs \Pipar 1 \nupar +  \Dy h \nuper  -  \tildev - \eps_0 \odelta \|_2^2 +  \frac{1}{n} \sum_{i=1}^n \lossf(\tilde{v}_i) \\
    \overset{\tildev = v - \eps\odelta}{=} &\min_{\tildev}~ \frac{1}{n} \sum_{i=1}^n \frac{\orv}{2\tau n} \left((\Dy \Xs \Pipar 1 \nupar)_i +  (\Dy h \nuper)_i  -  \tildev_i - \eps_0 \odelta \right)^2 +   \lossf(\tilde{v}_i) \\
  \overset{\mathrm{LLN}}{\to} &~~\EE_{\Zpar,\Zperp}\left[ \Moreau_{\lossf}(\abs{\Zpar}\nupar + \Zperp \nuper - \eps_0 \odelta, \frac{\tau}{\orv})\right],
\end{align*}
 where in the last line we used that $(\Dy\Xs \Pipar \Piper1)_i = \y_i\x_i^\top\thetanull = \xi_{\sigma}\sgn(\x_i^\top\thetanull) \x_i^\top\thetanull$ which has the same distribution as $\abs{\Zpar}$. Further, to apply the law of large numbers, we need to show that the Moreau envelope exists. Similarly to Theorem 1 \cite{Salehi19}, this follows immediately when noting that ${\Moreau_{\lossf}(x,\mu) \leq \lossf(x) = \log(1+\exp(-x)) \leq \log(2) + \abs{x}}$.
Finally, we obtain the desired optimization problem when combining these results.

\paragraph{Uniform convergences}
So far, we only proved point wise convergence to the same solution of the primal \ref{eq:thmnonsepridge} and auxiliary \ref{eq:nonseperable} optimization problem. However, since we also optimize over $v$, we need to show uniform convergence to guarantee that the solutions are asymptotically the same. This follows when using similar arguments as in Lemma A.5 \cite{Thrampoulidis15}.
Finally, note that the optima $\delta^\star$ in Equation \eqref{eq:delta} satisfies $\delta^\star = \frac{1}{\sqrt{d}} \| \Piper \theta\|$, and similarly the optima $\nuper^\star$ and $\nupar^\star$ in Equation \eqref{eq:nuperpar} satisfy $\nuper^\star = \| \Piper \theta\|_2$ and $\nupar^\star = \langle \theta,  \thetanull \rangle$. Hence we can conclude the proof as the solutions \ref{eq:nonseperable}, \eqref{eq:thmnonsepridge} 
converge asymptotically to the same optima.
%\qed

 \subsection{Proof of Theorem \ref{thm:seperable}}
 \label{sec:proofseperable}
 The proof is similar to the proof of  Theorem 6.3 \cite{Javanmard20b}.  
Recall the penalized max margin solution form Equation \eqref{eq:maxmarginAE}:
\begin{equation}
\label{eq:f5proofmaxma}
   \min_{\theta} \|\theta\|_2^2 ~~\mathrm{sucht~that~forall~}i: \langle \theta, \x_i \rangle - \eps \|\Piper \theta\|_1 \geq 1
  \end{equation}
When introducing the Lagrange multiplier $\zeta$ and $u$ we can write equivalently write:
  \begin{equation*}
   \min_{\theta, \delta}\max_{\substack{u: u_i\geq 0, \\ \zeta\geq 0}}
   \|\theta\|_2^2 + \frac{1}{n}u^\top \left( 1 + 1 \eps_0 \delta - D_y \Xs \theta\right) + \zeta(\frac{\| \Piper \theta\|_1}{\sqrt{d}} -\delta). 
   \end{equation*}
   and separating $\Xs$ again into $\Xs \Piper + \Xs \Pipar$, we get
   \begin{equation}
   \label{eq:primalsep}
      \min_{\theta, \delta}\max_{\substack{u: u_i\geq 0, \\ \zeta\geq 0}}
   \|\theta\|_2^2 + \frac{1}{n}u^\top \left( 1 + 1 \eps_0 \delta - D_y \Xs \Pipar \theta - D_y \Xs \Piper \theta \right) + \zeta(\frac{\|\Piper \theta\|_1}{\sqrt{d}} -\delta) 
     \end{equation}
\paragraph{Convex Gaussian Minimax Theorem}
     Since the adversarial attacks are consistent and the observations are noiseless, we know the solution in Equation \eqref{eq:f5proofmaxma} exists for all $d,n$. Yet, in order to apply the CGMT, we have to show that we can restrict $u$ and $\theta$ to compact sets. This follows for a simple trick as explained in Section D.3.1 \cite{Javanmard20b}. Hence, the primal optimization problem from Equation \eqref{eq:primalsep} can be asymptotically replaced with the following auxiliary optimization:
     \begin{equation*}
  \begin{split}
      &\min_{\theta, \delta}\max_{\substack{u: u_i\geq 0, \\ \zeta\geq 0}}
   \|\theta\|_2^2 + \frac{1}{n}u^\top \left( 1 + 1 \eps_0 \delta - D_y \Xs \Pipar \theta + D_y h \|\Piper \theta\|_2 \right) + \frac{1}{n}\|u\|_2  g^\top \Piper \theta + \zeta\left(\frac{\|\Piper \theta\|_1}{\sqrt{d}} -\delta\right) \\
   \end{split}
     \end{equation*}
     \paragraph{Scalarization of the optimization problem}
     The goal is again to scalarize the optimization problem. As a first step, we can solve the optimization over $u$ when defining $r = \frac{\|u\|_2}{\sqrt{n}}$: 
    \begin{equation*}
  \begin{split}
      \min_{\theta, \delta}\max_{\substack{r\geq 0, \\ \zeta\geq 0}}
   &\|\theta\|_2^2 + \frac{r}{\sqrt{n}}\| \max\left(0, 1 + 1 \eps_0 \delta - D_y \Xs \Pipar \theta + D_y h \|\Piper \theta\|_2 \right)\|_2 \\
   + &\frac{r\sqrt{\gamma}}{\sqrt{d}}\|u\|_2  g^\top \Piper \theta + \zeta\left( \frac{1}{\sqrt{d}}\|\Piper \theta\|_1 -\delta\right),
   \end{split}
     \end{equation*}
where $\max$ is taken elementwise over the vector. We now want to separate $\|\Piper \theta\|_2$ form the term in $\max(.)$. This is achieved by introducing the variables $\nuper \geq 0$ and the Lagrange multiplier $\kappa$. Further, we set $\nupar = \langle \thetastar, \Pipar \theta\rangle$, which allows us to equivalently write 
    \begin{equation*}
  \begin{split}
      \min_{\substack{\nuper\geq 0, \\ \nupar, \delta}}\max_{\substack{r\geq 0, \\ \zeta\geq 0, \kappa}}
   & \nupar^2  +\|\Piper \theta\|_2^2 +\kappa(\|\Piper \theta\|_2^2 - \nuper^2) + \frac{r}{\sqrt{n}}\| \max\left(0, 1 + 1 \eps_0 \delta - D_y \Xs \Pipar \theta_0 \nupar + D_y h \nuper \right)\|_2 \\
   + &\frac{r\sqrt{\gamma}}{\sqrt{d}}\|u\|_2  g^\top \Piper \theta +  \zeta\left(\frac{1}{\sqrt{d}}\|\Piper \theta\|_1 -\delta\right)
   \end{split}
     \end{equation*}
We further note that
     \begin{align*}
 &\frac{r}{\sqrt{n}}\| \max\left(0, 1 + 1 \eps_0 \delta - D_y \Xs \Pipar \theta_0 \nupar + D_y h \nuper \right)\|_2 \\ \overset{\mathrm{LLN}}{\to}~ &r \sqrt{\EE_{\Zpar,\Zperp} \left[\max\left(0,1+\eps_0\delta - \abs{\Zpar} \nupar + \Zperp \nuper\right)^2\right]} =: \sqrt{T}.
\end{align*}

% Further, we can extend the formula to:
%     \begin{equation}
%   \begin{split}
%       \min_{\nuper\geq 0,\nupar, \delta,\otaur \geq 0}\max_{r\geq 0, \zeta\geq 0, \kappa}
%    \nupar^2  + \|\Piper \theta\|_2^2 +\frac{\kappa}{2\otaur} \|\Piper \theta\|_2^2 + \frac{\kappa \otaur}{2} -\kappa\nuper + T
%    + \frac{r\sqrt{\gamma}}{\sqrt{d}}\|u\|_2  g^\top \Piper \theta + \zeta(\frac{\|\Piper \theta\|_1}{\sqrt{d}} -\delta) 
%    \end{split}
%      \end{equation}
Next, by completion of the squares we get
    \begin{equation*}
  \begin{split}
      \min_{\substack{ \nuper\geq 0, \\\nupar, \delta}}\max_{\substack{r\geq 0, \\ \zeta\geq 0, \kappa}}
   &\nupar^2  + (1+\kappa)\|\Piper \theta + \frac{r \sqrt{\gamma}}{\sqrt{d} 2(1+\kappa)} g\|_2^2 - \frac{r^2 \gamma}{ 4 (1+\kappa)} \|g/\sqrt{d}\|_2^2
   \\
   & -\kappa\nuper^2 + \sqrt{T} +\zeta  \left(\frac{1}{\sqrt{d}}\|\Piper \theta\|_1 -\delta\right), 
   \end{split}
     \end{equation*}
with $\|g/\sqrt{d}\|_2^2 \to 1$. Hence, it only remains to solve the inner optimization over $\Piper \theta$. We can write:
\begin{equation*}
\begin{split}
 \min_{\Piper \theta}~&(1+\kappa)\|\Piper \theta + \frac{r \sqrt{\gamma}}{\sqrt{d} 2(1+\kappa)} g\|_2^2 + \zeta \frac{\|\Piper \theta\|_1}{\sqrt{d}}  \\
 \overset{\tilde{\theta}_{\perp} = \frac{\Piper \theta}{\sqrt{d}}}= \min_{\tilde{\theta}_{\perp}} &\frac{1}{d} (1+\kappa)\| \tilde{\theta}_{\perp} +\frac{r \sqrt{\gamma}}{2(1+\kappa)} g \| + \zeta \frac{\|\Piper \theta\|_1}{d}
 \\ = &\frac{1}{d} \sum_{i=2}^d  \min_{(\tilde{\theta}_{\perp})_i}~ (1+\kappa)((\tilde{\theta}_{\perp})_i +\frac{r \sqrt{\gamma}}{ 2(1+\kappa)} g_i)^2 +  \zeta \abs{(\tilde{\theta}_{\perp})_i}
   \\ = &\frac{1}{d} 2(1+\kappa) \sum_{i=2}^d  \min_{(\tilde{\theta}_{\perp})_i}~ \frac{1}{2}((\tilde{\theta}_{\perp})_i +\frac{r \sqrt{\gamma}}{ 2(1+\kappa)} g_i)^2 + \frac{\zeta}{2(1+\kappa)} \abs{(\tilde{\theta}_{\perp})_i}
    \\ = &\frac{1}{d} 2(1+\kappa) \sum_{i=2}^d  \huberloss(-\frac{r \sqrt{\gamma}}{ 2(1+\kappa)} g_i, \frac{\zeta}{2(1+\kappa)})
\\ \to  & 2(1+\kappa) \EE_Z ~\huberloss \left(\frac{r \sqrt{\gamma}}{ 2(1+\kappa)} Z, \frac{\zeta}{2(1+\kappa)}\right)
 \end{split}
\end{equation*}
where $\huberloss$ is the Huber loss, given by $\huberloss(x,y) = \left\{ \begin{matrix} 0.5 x^2 ~~\abs{x} \leq y \\ y (\abs{x} - 0.5 y)                                                                                       \end{matrix} \right.$. Finally, we can conclude the proof from 
\begin{equation*}
 \EE_Z ~\huberloss \left(a Z, b\right) =  \frac{a^2+b^2}{2}\erf\left(\frac{b}{\sqrt{2} a}\right) - \frac{b^2}{2} + \frac{a b}{\sqrt{2 \pi}} \exp\left(- \frac{b^2}{2 a^2} \right) 
\end{equation*}
